# Supplementary material for: Dealing with Drift of Adaptation Spaces in Learning-based Self-Adaptive Systems using Lifelong Self-Adaptation
Source: arXiv:2211.02658 source file (2024-01-13)
Supplement: Supplementary file 1 [file appendix_2_old.tex]

\re{
\section{Statistical Test Results}
\label{sec: appendix statistical test results}
}

%\re{
In this section, we report statistical test results for a set of hypotheses used in the paper's main text, corresponding to each figure containing a set of box plots.  We limit the tests to the relevant results. 


\subsection{Quality Properties of Lifelong Self-Adaptation (Figure~\ref{fig:compare performance on quality attributes})}
Figure~\ref{fig:compare performance on quality attributes} illustrates the quality properties of lifelong self-adaptation compared to the other approaches for the base scenario. We have the following set of null hypotheses related to this figure where $\mu_{i,j,k}$ represents the mean of distribution for an attribute $j$. Possible values for $j$ are $p$ and $e$ representing packet loss and energy consumption, respectively. $i$ in $\mu_{i,j,k}$ refers to the scenario, that is, $n$ means a scenario without drift and $d$ means a scenario with drift, i.e., novel class appearance. Finally, $k$ in $\mu_{i,j,k}$  indicates the approach that has been used.

\begin{itemize}

    \retwo{
    \item The four approaches perform equally well for the quality attributes, i.e., packet loss and energy consumption, without drift of adaptation spaces:
    
    \begin{align*}
        H_0: & \mu_{n, p,\text{baseline}} = \mu_{n, p,\text{ML2ASR}}, \mu_{n, p,\text{baseline}} = \mu_{n, p,\text{LSA}}, \mu_{n, p,\text{baseline}}= \mu_{n, p,\text{LSA\_with\_op}}, \\ 
        &\mu_{n, p,\text{ML2ASR}} = \mu_{n, p,\text{LSA}},  \mu_{n, p,\text{ML2ASR}} = \mu_{n, p,\text{LSA\_with\_op}}, \mu_{n, p,\text{LSA}}= \mu_{n, p,\text{LSA\_with\_op}}, \\
        & \mu_{n, e,\text{baseline}} = \mu_{n, e,\text{ML2ASR}}, \mu_{n, e,\text{baseline}} = \mu_{n, e,\text{LSA}}, \mu_{n, p,\text{baseline}}= \mu_{n, e,\text{LSA\_with\_op}}, \\ &\mu_{n, e,\text{ML2ASR}} = \mu_{n, e,\text{LSA}},  \mu_{n, e,\text{ML2ASR}} = \mu_{n, e,\text{LSA\_with\_op}}, \mu_{n, e,\text{LSA}}= \mu_{n, e,\text{LSA\_with\_op}}
    \end{align*}
    }
    % \item Regarding the quality attributes, the evolving classifier with LSA with operator feedback performs as well as the baseline:
    \item The evolving classifier with LSA with operator feedback and the baseline perform equally well for the quality attributes with drift of adaptation spaces:
    \begin{align*}
        H_0: & \mu_{d, p,\text{baseline}} = \mu_{d,p,\text{LSA\_with\_op}} \text{ and } \mu_{d,e,\text{baseline}} = \mu_{d,e,\text{LSA\_with\_op}}
    \end{align*}

    % \item Regarding the energy consumption, the predefined classifier with LSA (no operator feedback) performs as well as the baseline:
    % \item The predefined classifier with LSA (no operator feedback) performs as well as the baseline for the quality attributes with drift of adaptation spaces:
    % \begin{align*}
    %     H_0: & \mu_{d, e,\text{baseline}} = \mu_{d,e,\text{LSA}} \\ 
    %     H_1: & \mu_{d,e,\text{baseline}} < \mu_{d,e,\text{LSA}}
    % \end{align*}

    % \item Regarding the energy consumption, the predefined classifier with ML2ASR performs as well as the baseline:
    % \begin{align*}
    %     H_0: & \mu_{d, e,\text{baseline}} = \mu_{d,e,\text{ML2ASR}} \\ 
    %     H_1: & \mu_{d,e,\text{baseline}} < \mu_{d,e,\text{ML2ASR}}
    % \end{align*}
\end{itemize}

%Note that when we do not explicitly mention an alternative hypothesis for an equality hypothesis, the alternative would be two-sided, i.e., inequality of the corresponding means. 

To test these hypotheses, we start with determining an appropriate test method. As a start, we use the Anderson–Darling test~\cite{d2017goodness} to test whether the data of packet loss and energy consumption are normally distributed in different box plots. Based on the results of Table~\ref{tab: normality test fig 19}, with a significance level ($\alpha$) of $0.05$, all normality tests are rejected. 


\begin{table}[h]
\center
\begin{tabular}{c|c|c|c|}
\cline{2-4}
\multicolumn{1}{l|}{}                                       & Approach          & \begin{tabular}[c]{@{}c@{}}p-value \\ Anderson-Darling test \\ (packet loss)\end{tabular} & \begin{tabular}[c]{@{}c@{}}p-value \\ Anderson-Darling test \\ (energy consumption)\end{tabular} \\ \hhline{-===}
\multicolumn{1}{|c|}{\multirow{4}{*}{no drift}}             & Baseline          & \reject{0.000} & \reject{0.000}                        \\ \cline{2-4} 
\multicolumn{1}{|c|}{}                                      & ML2ASR            & \reject{0.000} & \reject{0.000}                         \\ \cline{2-4} 
\multicolumn{1}{|c|}{}                                      & LSA               & \reject{0.000} & \reject{0.000}                         \\ \cline{2-4} 
\multicolumn{1}{|c|}{}                                      & LSA with operator & \reject{0.000} & \reject{0.000}                         \\ \hhline{====}
\multicolumn{1}{|c|}{\multirow{2}{*}{\begin{tabular}[c]{@{}c@{}}novel class \\ appeared\end{tabular}}} & Baseline          & \reject{0.000} & \reject{0.000}                         \\ \cline{2-4} 
%\multicolumn{1}{|c|}{}                                      & ML2ASR            & \reject{0.005} & \reject{0.006}                         \\ \cline{2-4} 
% \multicolumn{1}{|c|}{}                                      & LSA               & \reject{0.048} & \reject{0.002}                         
%\\ \cline{2-4} 
\multicolumn{1}{|c|}{}                                      & LSA with operator & \reject{0.000} & \reject{0.000}                        
\\ \hline
\end{tabular}

\caption{\re{Normality test for packet loss and energy consumption values in Figure~\ref{fig:compare performance on quality attributes}. }} 
\label{tab: normality test fig 19}
\end{table}

% \begin{table}[h]
% \center
% \begin{subtable}[t]{0.48\textwidth}
% \center
% \begin{adjustbox}{max width=\textwidth}
% \begin{tabular}{c|c|c|}
% \cline{2-3}
% \multicolumn{1}{l|}{}                                       & Approach          & \begin{tabular}[c]{@{}c@{}}p-value \\ Anderson-Darling test\end{tabular} \\ \hline
% \multicolumn{1}{|c|}{\multirow{4}{*}{no drift}}             & Baseline          & \reject{0.000}                         \\ \cline{2-3} 
% \multicolumn{1}{|c|}{}                                      & ML2ASR            & \reject{0.000}                         \\ \cline{2-3} 
% \multicolumn{1}{|c|}{}                                      & LSA               & \reject{0.000}                         \\ \cline{2-3} 
% \multicolumn{1}{|c|}{}                                      & LSA with operator & \reject{0.000}                         \\ \hline
% \multicolumn{1}{|c|}{\multirow{4}{*}{\begin{tabular}[c]{@{}c@{}}novel class \\ appeared\end{tabular}}} & Baseline          & \reject{0.000}                         \\ \cline{2-3} 
% \multicolumn{1}{|c|}{}                                      & ML2ASR            & 0.005                         \\ \cline{2-3} 
% \multicolumn{1}{|c|}{}                                      & LSA               & 0.048                         \\ \cline{2-3} 
% \multicolumn{1}{|c|}{}                                      & LSA with operator & \reject{0.000}                         \\ \hline
% \end{tabular}
% \end{adjustbox}
% \caption{packet loss}
% \end{subtable}
% \begin{subtable}[t]{0.48\textwidth}
% \center
% \begin{adjustbox}{max width=\textwidth}
% \begin{tabular}{c|c|c|}
% \cline{2-3}
% \multicolumn{1}{l|}{}                                       & Approach          & \begin{tabular}[c]{@{}c@{}}p-value \\ Anderson-Darling test\end{tabular} \\ \hline
% \multicolumn{1}{|c|}{\multirow{4}{*}{no drift}}             & Baseline          & \reject{0.000}                         \\ \cline{2-3} 
% \multicolumn{1}{|c|}{}                                      & ML2ASR            & \reject{0.000}                         \\ \cline{2-3} 
% \multicolumn{1}{|c|}{}                                      & LSA               & \reject{0.000}                         \\ \cline{2-3} 
% \multicolumn{1}{|c|}{}                                      & LSA with operator & \reject{0.000}                         \\ \hline
% \multicolumn{1}{|c|}{\multirow{4}{*}{\begin{tabular}[c]{@{}c@{}}novel class \\ appeared\end{tabular}}} & Baseline          & \reject{0.000}                         \\ \cline{2-3} 
% \multicolumn{1}{|c|}{}                                      & ML2ASR            & 0.006                         \\ \cline{2-3} 
% \multicolumn{1}{|c|}{}                                      & LSA               & 0.002                         \\ \cline{2-3} 
% \multicolumn{1}{|c|}{}                                      & LSA with operator & \reject{0.000}                         \\ \hline
% \end{tabular}
% \end{adjustbox}
% \caption{energy consumption}
% \end{subtable}
% \caption{\re{Normality test for packet loss and energy consumption values in Figure~\ref{fig:compare performance on quality attributes}. }} 
% \label{tab: normality test fig 19 }
% \end{table}

%The dependency of the data is another critical factor in choosing a proper statistical test method. 
As all normality tests are rejected, we can use the Spearman correlation method~\cite{myers2010research} to test whether each pair of data for the relevant corresponding approaches is dependent. Table~\ref{tab: dependency test fig 19} shows, with a significance level ($\alpha$) of $0.05$, that all pairs for both attributes are independent (i.e., all null hypotheses have been rejected). 
%except pairs of (Baseline, ML2ASR), (Baseline, LSA), (ML2ASR, LSA), (ML2ASER, LSA with operator), and(LSA, LSA with operator) in the packet loss when novel class appeared. 
Based on the results of the normality tests and the dependency tests, we used Mann-Whitney U test~\cite{MacFarland2016} as test methods for the data of Figure~\ref{fig:compare performance on quality attributes}. 
%two non-parametric statistical tests: the Wilcoxon signed-rank test~\cite{conover1980practical} for dependent pairs and the Mann-Whitney U test~\cite{MacFarland2016} for others.

\begin{table}[h]
\center
\begin{adjustbox}{max width=\textwidth}
\begin{tabular}{c|c|c|c|}
\cline{2-4}
\multicolumn{1}{l|}{}                                       & Approach Pair          & \begin{tabular}[c]{@{}c@{}}p-value \\ Spearman correlation test \\ (packet loss)\end{tabular} & \begin{tabular}[c]{@{}c@{}}p-value \\ Spearman correlation test \\ (energy consumption)\end{tabular} \\ \hhline{-===}
\multicolumn{1}{|c|}{\multirow{6}{*}{no drift}}             & (Baseline, ML2ASR)          & \reject{0.000} & \reject{0.000}                         \\ \cline{2-4} 
\multicolumn{1}{|c|}{}                                      & (Baseline, LSA)            & \reject{0.000} & \reject{0.000}                        \\ \cline{2-4} 
\multicolumn{1}{|c|}{}                                      & (Baseline, LSA with operator)               & \reject{0.000} & \reject{0.000}                         \\ \cline{2-4} 
\multicolumn{1}{|c|}{}                                      & (ML2ASR, LSA)               & \reject{0.000} & \reject{0.000}                        \\ \cline{2-4} 
\multicolumn{1}{|c|}{}                                      & (ML2ASR, LSA with operator)               & \reject{0.000} & \reject{0.000}                        \\ \cline{2-4} 
\multicolumn{1}{|c|}{}                                      & (LSA, LSA with operator) & \reject{0.000} & \reject{0.000}                         \\ \hhline{====}
% \multicolumn{1}{|c|}{\multirow{1}{*}{\begin{tabular}[c]{@{}c@{}}novel class \\ appeared\end{tabular}}} 

\multicolumn{1}{|c|}{{\begin{tabular}[c]{@{}c@{}}novel class \\ appeared\end{tabular}}} 

% & (Baseline, ML2ASR)          & \accept{0.234} & \reject{0.000}                         \\ \cline{2-4} 
% \multicolumn{1}{|c|}{}                                      
%& (Baseline, LSA)            & \accept{0.686} & \reject{0.000}                         %\\ \cline{2-4} 
% \multicolumn{1}{|c|}{}
& (Baseline, LSA with operator)               & \reject{0.000} & \reject{0.000}                         %\\ \cline{2-4} 
% \multicolumn{1}{|c|}{}                                      & (ML2ASR, LSA)               & \accept{0.815} & \reject{0.000}                         \\ \cline{2-4} 
% \multicolumn{1}{|c|}{}                                      & (ML2ASR, LSA with operator)               & \accept{0.508} & \reject{0.000}                        \\ \cline{2-4} 
% \multicolumn{1}{|c|}{}                                      & (LSA, LSA with operator) & \accept{0.506}   & \reject{0.000}                      
\\ \hline
\end{tabular}
\end{adjustbox}
\caption{\re{Dependency test for packet loss and energy consumption values in Figure~\ref{fig:compare performance on quality attributes}. }} 
\label{tab: dependency test fig 19}
\end{table}

% \begin{table}[h]
% \center
% \begin{subtable}[t]{0.48\textwidth}
% \center
% \begin{adjustbox}{max width=\textwidth}
% \begin{tabular}{c|c|c|}
% \cline{2-3}
% \multicolumn{1}{l|}{}                                       & Approach Pair          & \begin{tabular}[c]{@{}c@{}}p-value \\ Spearman correlation test\end{tabular} \\ \hline
% \multicolumn{1}{|c|}{\multirow{6}{*}{no drift}}             & (Baseline, ML2ASR)          & \reject{0.000}                         \\ \cline{2-3} 
% \multicolumn{1}{|c|}{}                                      & (Baseline, LSA)            & \reject{0.000}                         \\ \cline{2-3} 
% \multicolumn{1}{|c|}{}                                      & (Baseline, LSA with operator)               & \reject{0.000}                         \\ \cline{2-3} 
% \multicolumn{1}{|c|}{}                                      & (ML2ASR, LSA)               & \reject{0.000}                         \\ \cline{2-3} 
% \multicolumn{1}{|c|}{}                                      & (ML2ASR, LSA with operator)               & \reject{0.000}                         \\ \cline{2-3} 
% \multicolumn{1}{|c|}{}                                      & (LSA, LSA with operator) & \reject{0.000}                         \\ \hline
% \multicolumn{1}{|c|}{\multirow{6}{*}{\begin{tabular}[c]{@{}c@{}}novel class \\ appeared\end{tabular}}}             & (Baseline, ML2ASR)          & 0.234                         \\ \cline{2-3} 
% \multicolumn{1}{|c|}{}                                      & (Baseline, LSA)            & 0.686                         \\ \cline{2-3} 
% \multicolumn{1}{|c|}{}                                      & (Baseline, LSA with operator)               & \reject{0.000}                         \\ \cline{2-3} 
% \multicolumn{1}{|c|}{}                                      & (ML2ASR, LSA)               & 0.815                         \\ \cline{2-3} 
% \multicolumn{1}{|c|}{}                                      & (ML2ASR, LSA with operator)               & 0.508                         \\ \cline{2-3} 
% \multicolumn{1}{|c|}{}                                      & (LSA, LSA with operator) & 0.506                         \\ \hline
% \end{tabular}
% \end{adjustbox}
% \caption{packet loss}
% \end{subtable}
% \begin{subtable}[t]{0.48\textwidth}
% \center
% \begin{adjustbox}{max width=\textwidth}
% \begin{tabular}{c|c|c|}
% \cline{2-3}
% \multicolumn{1}{l|}{}                                       & Approach Pair          & \begin{tabular}[c]{@{}c@{}}p-value \\ Spearman correlation test\end{tabular} \\ \hline
% \multicolumn{1}{|c|}{\multirow{6}{*}{no drift}}             & (Baseline, ML2ASR)          & \reject{0.000}                         \\ \cline{2-3} 
% \multicolumn{1}{|c|}{}                                      & (Baseline, LSA)            & \reject{0.000}                         \\ \cline{2-3} 
% \multicolumn{1}{|c|}{}                                      & (Baseline, LSA with operator)               & \reject{0.000}                         \\ \cline{2-3} 
% \multicolumn{1}{|c|}{}                                      & (ML2ASR, LSA)               & \reject{0.000}                         \\ \cline{2-3} 
% \multicolumn{1}{|c|}{}                                      & (ML2ASR, LSA with operator)               & \reject{0.000}                         \\ \cline{2-3} 
% \multicolumn{1}{|c|}{}                                      & (LSA, LSA with operator) & \reject{0.000}                         \\ \hline
% \multicolumn{1}{|c|}{\multirow{6}{*}{\begin{tabular}[c]{@{}c@{}}novel class \\ appeared\end{tabular}}}             & (Baseline, ML2ASR)          & \reject{0.000}                         \\ \cline{2-3} 
% \multicolumn{1}{|c|}{}                                      & (Baseline, LSA)            & \reject{0.000}                         \\ \cline{2-3} 
% \multicolumn{1}{|c|}{}                                      & (Baseline, LSA with operator)               & \reject{0.000}                         \\ \cline{2-3} 
% \multicolumn{1}{|c|}{}                                      & (ML2ASR, LSA)               & \reject{0.000}                         \\ \cline{2-3} 
% \multicolumn{1}{|c|}{}                                      & (ML2ASR, LSA with operator)               & \reject{0.000}                         \\ \cline{2-3} 
% \multicolumn{1}{|c|}{}                                      & (LSA, LSA with operator) & \reject{0.000}                         \\ \hline
% \end{tabular}
% \end{adjustbox}
% \caption{energy consumption}
% \end{subtable}
% \caption{\re{Dependency test for packet loss and energy consumption values in Figure~\ref{fig:compare performance on quality attributes}. }} 
% \label{tab: dependency test fig 19 }
% \end{table}


% As we found different circumstances for each pair of equality hypothesis in $H_0$s, each pair was tested based on its proper statistical test method with a corrected significance level of $0.05$, by the Bonferroni method (i.e., all p-values were multiplied by the number of pairs of equalities in the corresponding hypothesis). The details of the test results for each hypothesis are in the following two tables (i.e., Table~\ref{tab: hypothesis 1 test fig 19} and \ref{tab: hypothesis 2 test fig 19}).

\retwo{
The details of the test results for each hypothesis are in the following two tables (i.e., Table~\ref{tab: hypothesis 1 test fig 19} and \ref{tab: hypothesis 2 test fig 19}). Regarding the concern of the Bonferroni correction method, all p-values were multiplied by the number of pairs of equalities in the corresponding hypothesis, i.e., keeping the significance level at 0.05 without any change.
}

\begin{table}[h]
\center
% \begin{subtable}[t]{0.48\textwidth}
% \center
% \begin{adjustbox}{max width=\textwidth}
% \begin{tabular}{|c|c|c|}
% \hline
%  Hypothesis & p-value & Test method \\ \hhline{===}
%  $\mu_{n, p,\text{baseline}} = \mu_{n, p,\text{ML2ASR}}$ & \reject{0.001} & Mann-Whitney U \\ \hline
%  $\mu_{n, p,\text{baseline}} = \mu_{n, p,\text{LSA}}$& \accept{0.159} & Mann-Whitney U \\ \hline
% $\mu_{n, p,\text{baseline}} = \mu_{n, p,\text{LSA\_with\_op}}$& \accept{0.052} & Mann-Whitney U \\ \hline
% $\mu_{n, p,\text{ML2ASR}} = \mu_{n, p,\text{LSA}}$& \accept{0.643} & Mann-Whitney U  \\ \hline
% $\mu_{n, p,\text{ML2ASR}} = \mu_{n, p,\text{LSA\_with\_op}}$& \accept{1.000} &  Mann-Whitney U\\ \hline
% $\mu_{n, p,\text{LSA}} = \mu_{n, p,\text{LSA\_with\_op}}$& \accept{1.000} & Mann-Whitney U \\ \hline
% \end{tabular}
% \end{adjustbox}
% \caption{packet loss}
% \end{subtable}
% \begin{subtable}[t]{0.48\textwidth}
% \center
% \begin{adjustbox}{max width=\textwidth}
% \begin{tabular}{|c|c|c|}
% \hline
%  Hypothesis & p-value & Test method \\ \hhline{===}
%  $\mu_{n, e,\text{baseline}} = \mu_{n, e,\text{ML2ASR}}$ & \reject{0.006} &  Mann-Whitney U\\ \hline
%  $\mu_{n, e,\text{baseline}} = \mu_{n, e,\text{LSA}}$& \accept{1.000} & Mann-Whitney U \\ \hline
% $\mu_{n, e,\text{baseline}} = \mu_{n, e,\text{LSA\_with\_op}}$& \accept{1.000} & Mann-Whitney U \\ \hline
% $\mu_{n, e,\text{ML2ASR}} = \mu_{n, e,\text{LSA}}$& \reject{0.048}  & Mann-Whitney U \\ \hline
% $\mu_{n, e,\text{ML2ASR}} = \mu_{n, e,\text{LSA\_with\_op}}$& \reject{0.008} & Mann-Whitney U \\ \hline
% $\mu_{n, e,\text{LSA}} = \mu_{n, e,\text{LSA\_with\_op}}$& \accept{1.000} & Mann-Whitney U \\ \hline
% \end{tabular}
% \end{adjustbox}
% \caption{energy consumption}
% \end{subtable}

\begin{subtable}[t]{0.48\textwidth}
\center
\begin{adjustbox}{max width=\textwidth}
\begin{tabular}{|c|c|c|}
\hline
 Hypothesis & p-value & Test method \\ \hhline{===}
 $\mu_{n, p,\text{baseline}} = \mu_{n, p,\text{ML2ASR}}$ & \reject{0.001} & Mann-Whitney U \\ \hline
 $\mu_{n, p,\text{baseline}} = \mu_{n, p,\text{LSA}}$& \accept{0.318} & Mann-Whitney U \\ \hline
$\mu_{n, p,\text{baseline}} = \mu_{n, p,\text{LSA\_with\_op}}$& \accept{0.105} & Mann-Whitney U \\ \hline
$\mu_{n, p,\text{ML2ASR}} = \mu_{n, p,\text{LSA}}$& \accept{1.000} & Mann-Whitney U  \\ \hline
$\mu_{n, p,\text{ML2ASR}} = \mu_{n, p,\text{LSA\_with\_op}}$& \accept{1.000} &  Mann-Whitney U\\ \hline
$\mu_{n, p,\text{LSA}} = \mu_{n, p,\text{LSA\_with\_op}}$& \accept{1.000} & Mann-Whitney U \\ \hline
\end{tabular}
\end{adjustbox}
\caption{packet loss}
\end{subtable}
\begin{subtable}[t]{0.48\textwidth}
\center
\begin{adjustbox}{max width=\textwidth}
\begin{tabular}{|c|c|c|}
\hline
 Hypothesis & p-value & Test method \\ \hhline{===}
 $\mu_{n, e,\text{baseline}} = \mu_{n, e,\text{ML2ASR}}$ & \reject{0.012} &  Mann-Whitney U\\ \hline
 $\mu_{n, e,\text{baseline}} = \mu_{n, e,\text{LSA}}$& \accept{1.000} & Mann-Whitney U \\ \hline
$\mu_{n, e,\text{baseline}} = \mu_{n, e,\text{LSA\_with\_op}}$& \accept{1.000} & Mann-Whitney U \\ \hline
$\mu_{n, e,\text{ML2ASR}} = \mu_{n, e,\text{LSA}}$& \accept{0.096}  & Mann-Whitney U \\ \hline
$\mu_{n, e,\text{ML2ASR}} = \mu_{n, e,\text{LSA\_with\_op}}$& \reject{0.017} & Mann-Whitney U \\ \hline
$\mu_{n, e,\text{LSA}} = \mu_{n, e,\text{LSA\_with\_op}}$& \accept{1.000} & Mann-Whitney U \\ \hline
\end{tabular}
\end{adjustbox}
\caption{energy consumption}
\end{subtable}



\caption{\re{Test results for the following null hypothesis: ``The four approaches perform equally well for the quality attributes, i.e., packet loss and energy consumption, without drift of adaptation spaces''.}}
\label{tab: hypothesis 1 test fig 19}
\end{table}


\begin{table}[h]
\center
% \begin{subtable}[t]{0.48\textwidth}
% \center
% \begin{adjustbox}{max width=\textwidth}
% \begin{tabular}{|c|c|c|}
% \hline
%  Hypothesis & p-value & Test method \\ \hhline{===}
% $\mu_{d, p,\text{baseline}} = \mu_{d, p,\text{LSA\_with\_op}}$ & \reject{0.027} & Mann-Whitney U \\ \hline
% \end{tabular}
% \end{adjustbox}
% \caption{packet loss}
% \end{subtable}
% \begin{subtable}[t]{0.48\textwidth}
% \center
% \begin{adjustbox}{max width=\textwidth}
% \begin{tabular}{|c|c|c|}
% \hline
%  Hypothesis & p-value & Test method \\ \hhline{===}
% $\mu_{d, e,\text{baseline}} = \mu_{d, e,\text{LSA\_with\_op}}$ & \accept{0.769} & Mann-Whitney U \\ \hline
% \end{tabular}
% \end{adjustbox}
% \caption{energy consumption}
% \end{subtable}

\begin{subtable}[t]{0.48\textwidth}
\center
\begin{adjustbox}{max width=\textwidth}
\begin{tabular}{|c|c|c|}
\hline
 Hypothesis & p-value & Test method \\ \hhline{===}
$\mu_{d, p,\text{baseline}} = \mu_{d, p,\text{LSA\_with\_op}}$ & \accept{0.060} & Mann-Whitney U \\ \hline
\end{tabular}
\end{adjustbox}
\caption{packet loss}
\end{subtable}
\begin{subtable}[t]{0.48\textwidth}
\center
\begin{adjustbox}{max width=\textwidth}
\begin{tabular}{|c|c|c|}
\hline
 Hypothesis & p-value & Test method \\ \hhline{===}
$\mu_{d, e,\text{baseline}} = \mu_{d, e,\text{LSA\_with\_op}}$ & \accept{1.000} & Mann-Whitney U \\ \hline
\end{tabular}
\end{adjustbox}
\caption{energy consumption}
\end{subtable}


\caption{\retwo{Test results for these null hypotheses: ``The evolving classifier with LSA with operator feedback performs as well as the baseline for the quality attributes with drift of adaptation spaces''.}}
\label{tab: hypothesis 2 test fig 19}
\end{table}

% \begin{table}[h]
% \center
% \begin{adjustbox}{max width=\textwidth}
% \begin{tabular}{|c|c|c|}
% \hline
%  Hypothesis & p-value & Test method \\ \hhline{===}
% \begin{tabular}[c]{@{}c@{}}
% $H_0: \mu_{d, e,\text{baseline}} = \mu_{d,e,\text{LSA}}$ \\ 
% $H_1: \mu_{d,e,\text{baseline}} < \mu_{d,e,\text{LSA}}$
% \end{tabular} & \reject{0.000} & Wilcoxon signed-rank
% \\ \hline
% \end{tabular}
% \end{adjustbox}
% \caption{\re{Test results for this null hypothesis: ``Regarding the energy consumption, the predefined classifier with LSA (no operator feedback) performs as well as the baseline''}}
% \label{tab: hypothesis 3 figure 21}
% \end{table}


% \begin{table}[h]
% \center
% \begin{adjustbox}{max width=\textwidth}
% \begin{tabular}{|c|c|c|}
% \hline
%  Hypothesis & p-value & Test method \\ \hhline{===}
% \begin{tabular}[c]{@{}c@{}}
% $H_0: \mu_{d, e,\text{baseline}} = \mu_{d,e,\text{ML2ASR}}$ \\ 
% $H_1: \mu_{d,e,\text{baseline}} < \mu_{d,e,\text{ML2ASR}}$
% \end{tabular} & \reject{0.000} & Wilcoxon signed-rank
% \\ \hline
% \end{tabular}
% \end{adjustbox}
% \caption{\re{Test results for this null hypothesis: ``Regarding the energy consumption, the predefined classifier with ML2ASR performs as well as the baseline''}}
% \label{tab: hypothesis 4 figure 21}
% \end{table}

\subsection{Impact of Drift of Adaptation Spaces on The Utility (Figure~\ref{fig:resuls-utilities})}
Figure~\ref{fig:resuls-utilities} illustrates the impact of drift of adaptation spaces on the utility of the system.
For the utility, we had the same hypotheses as packet loss and energy consumption. 
Here, we used the same notation as before, except using $u$ instead of $p$ or $e$ in $j$ index of $\mu_{i,j,k}$, to show that these means are related to the utility values. 
Accordingly, we have the following set of null hypotheses related to this figure.

\begin{itemize}
    \item The four approaches perform equally well for the utility without drift of adaptation spaces:
    \begin{align*}
        H_0: & \mu_{n, u,\text{baseline}} = \mu_{n, u,\text{ML2ASR}}, \mu_{n, u,\text{baseline}} = \mu_{n, u,\text{LSA}}, \mu_{n, u,\text{baseline}}= \mu_{n, u,\text{LSA\_with\_op}}, \\ &\mu_{n, u,\text{ML2ASR}} = \mu_{n, u,\text{LSA}},  \mu_{n, u,\text{ML2ASR}} = \mu_{n, u,\text{LSA\_with\_op}}, \mu_{n, u,\text{LSA}}= \mu_{n, u,\text{LSA\_with\_op}}
    \end{align*}
    
    % \item Regarding the utility value, the evolving classifier with LSA with operator feedback performs as well as the baseline:
    \item The evolving classifier with LSA with operator feedback performs as well as the baseline for the utility with drift of adaptation spaces:
    \begin{align*}
        H_0: & \mu_{d, u,\text{baseline}} = \mu_{d,u,\text{LSA\_with\_op}}
    \end{align*}
\end{itemize}



In the same process as the previous section, we tested first the normality of utilities, as its corresponding results are illustrated in Table~\ref{tab: normality test fig 20}. 
The results show that all normality tests have been rejected. 

\begin{table}[h]
\center
\begin{tabular}{c|c|c|}
\cline{2-3}
\multicolumn{1}{l|}{}                                       & Approach          & \begin{tabular}[c]{@{}c@{}}p-value \\ Anderson-Darling test\end{tabular} \\ \hhline{-==}
\multicolumn{1}{|c|}{\multirow{4}{*}{no drift}}             & Baseline          & \reject{0.000}                      \\ \cline{2-3} 
\multicolumn{1}{|c|}{}                                      & ML2ASR            & \reject{0.000}                       \\ \cline{2-3} 
\multicolumn{1}{|c|}{}                                      & LSA               & \reject{0.000}                         \\ \cline{2-3} 
\multicolumn{1}{|c|}{}                                      & LSA with operator & \reject{0.000}                       \\ \hhline{===}
\multicolumn{1}{|c|}{\multirow{4}{*}{\begin{tabular}[c]{@{}c@{}}novel class \\ appeared\end{tabular}}} & Baseline          & \reject{0.000}                          \\ \cline{2-3} 
\multicolumn{1}{|c|}{}                                      & ML2ASR            & \reject{0.000}                         \\ \cline{2-3} 
\multicolumn{1}{|c|}{}                                      & LSA               & \reject{0.000}                         \\ \cline{2-3} 
\multicolumn{1}{|c|}{}                                      & LSA with operator & \reject{0.000}                         \\ \hline
\end{tabular}

\caption{\re{Normality test for utility values in Figure~\ref{fig:resuls-utilities}.}} 
\label{tab: normality test fig 20}
\end{table}

As all normality null hypotheses were rejected (with a significant level of 0.05), we used the Spearman correlation test for the dependency test. The results are shown in Tabel~\ref{tab: dependency test fig 20}. This table shows that all dependency tests have also been rejected. 

\begin{table}[h]
\center
\begin{tabular}{c|c|c|}
\cline{2-3}
\multicolumn{1}{l|}{}                                       & Approach          & \begin{tabular}[c]{@{}c@{}}p-value \\ Spearman correlation test\end{tabular} \\ \hhline{-==}
\multicolumn{1}{|c|}{\multirow{6}{*}{no drift}}             & (Baseline, ML2ASR)          & \reject{0.000}                 \\ \cline{2-3} 
\multicolumn{1}{|c|}{}                                      & (Baseline, LSA)            & \reject{0.000}                        \\ \cline{2-3} 
\multicolumn{1}{|c|}{}                                      & (Baseline, LSA with operator)               & \reject{0.000}                          \\ \cline{2-3} 
\multicolumn{1}{|c|}{}                                      & (ML2ASR, LSA)               & \reject{0.000}                       \\ \cline{2-3} 
\multicolumn{1}{|c|}{}                                      & (ML2ASR, LSA with operator)               & \reject{0.000}                         \\ \cline{2-3} 
\multicolumn{1}{|c|}{}                                      & (LSA, LSA with operator) & \reject{0.000}                          \\ \hhline{===}

\multicolumn{1}{|c|}{\multirow{6}{*}{novel class appeared}}             & (Baseline, ML2ASR)          & \accept{0.085}                 \\ \cline{2-3} 
\multicolumn{1}{|c|}{}                                      & (Baseline, LSA)            & \accept{0.230}                        \\ \cline{2-3} 
\multicolumn{1}{|c|}{}                                      & (Baseline, LSA with operator)               & \reject{0.000}                          \\ \cline{2-3} 
\multicolumn{1}{|c|}{}                                      & (ML2ASR, LSA)               & \accept{0.940}                       \\ \cline{2-3} 
\multicolumn{1}{|c|}{}                                      & (ML2ASR, LSA with operator)               & \accept{0.936}                         \\ \cline{2-3} 
\multicolumn{1}{|c|}{}                                      & (LSA, LSA with operator) & \accept{0.083}                          \\ \hline
\end{tabular}

\caption{\re{Dependency test for utility values in Figure~\ref{fig:resuls-utilities}. }} 
\label{tab: dependency test fig 20}
\end{table}
 
Based on the dependency test results and rejection of all normality tests, we can find an appropriate test method among the two non-parametric methods: Mann-Whitney U and  Wilcoxon signed-rank methods; see Table~\ref{tab: hypothesis 1 test fig 20} and \ref{tab: hypothesis 2 test fig 20}.

\begin{table}[h]
\center
\begin{adjustbox}{max width=\textwidth}
\begin{tabular}{|c|c|c|}
\hline
 Hypothesis & p-value & Test method \\ \hhline{===}
 $\mu_{n, u,\text{baseline}} = \mu_{n, u,\text{ML2ASR}}$ & \reject{0.000} & Mann-Whitney U \\ \hline
 $\mu_{n, u,\text{baseline}} = \mu_{n, u,\text{LSA}}$& \accept{0.302} & Mann-Whitney U \\ \hline
$\mu_{n, u,\text{baseline}} = \mu_{n, u,\text{LSA\_with\_op}}$& \accept{0.254} & Mann-Whitney U \\ \hline
$\mu_{n, u,\text{ML2ASR}} = \mu_{n, u,\text{LSA}}$& \reject{0.043} & Mann-Whitney U  \\ \hline
$\mu_{n, u,\text{ML2ASR}} = \mu_{n, u,\text{LSA\_with\_op}}$& \reject{0.016} &  Mann-Whitney U\\ \hline
$\mu_{n, u,\text{LSA}} = \mu_{n, u,\text{LSA\_with\_op}}$& \accept{1.000} & Mann-Whitney U \\ \hline
\end{tabular}
\end{adjustbox}
\caption{\re{Test results for this null hypothesis: ``The four approaches perform equally well with regards to the utility without drift of adaptation spaces''}}
\label{tab: hypothesis 1 test fig 20}
\end{table}

\begin{table}[h]
\center
\begin{adjustbox}{max width=\textwidth}
\begin{tabular}{|c|c|c|}
\hline
 Hypothesis & p-value & Test method \\ \hhline{===}
$\mu_{d, u,\text{baseline}} = \mu_{d, u,\text{LSA\_with\_op}}$ & \accept{0.105} & Mann-Whitney U \\ \hline
\end{tabular}
\end{adjustbox}
\caption{\re{Test results for this null hypothesis: ``The evolving classifier with LSA with operator feedback performs as well as the baseline for the utility with drift of adaptation spaces''.}}
\label{tab: hypothesis 2 test fig 20}
\end{table}


\subsection{ Impact of Drift of Adaptation Spaces on The \rsm\ (Figure~\ref{fig: rsm improvement})}
\label{sec: appendix fig 21}

Figure~\ref{fig: rsm improvement} illustrates the impact of drift of adaptation spaces on the \rsm\ for different approaches. Because of no overlap between the corresponding box plot of ``LSA with the operator'' approach and other box plots when the novel class appeared, we do not have any statistical test regarding the improvement of \rsm\ value. However, we need to test their equality without drift of adaptation space, with the following null hypothesis:

\begin{itemize}
    \item The three approaches perform equally well with regards to \rsm\ without drift of adaptation spaces:
    \begin{align*}
        H_0: & \mu_{n, r,\text{ML2ASR}} = \mu_{n, r,\text{LSA}},  \mu_{n, r,\text{ML2ASR}} = \mu_{n, r,\text{LSA\_with\_op}}, \mu_{n, r,\text{LSA}}= \mu_{n, r,\text{LSA\_with\_op}}
    \end{align*}
\end{itemize}

\noindent
Here, we used the same notation as before, except using $r$ instead of $p$, $e$, or $u$ in $j$ index of $\mu_{i,j,k}$, to show that the mean is related to \rsm\ values.

Like previous cases, we first ran a method (using the Anderson-Darling method) to test normality in data. Table~\ref{tab: normality test fig 21} shows the corresponding results and indicates the rejection of the normality hypothesis for all distributions mapped to box plots. 


\begin{table}[h]
\center
\begin{tabular}{c|c|c|}
\cline{2-3}
\multicolumn{1}{l|}{}                                       & Approach          & \begin{tabular}[c]{@{}c@{}}p-value \\ Anderson-Darling test\end{tabular} \\ \hhline{-==}
\multicolumn{1}{|c|}{\multirow{4}{*}{no drift}}             & ML2ASR            & \reject{0.036}                       \\ \cline{2-3} 
\multicolumn{1}{|c|}{}                                      & LSA               & \reject{0.001}                         \\ \cline{2-3} 
\multicolumn{1}{|c|}{}                                      & LSA with operator & \reject{0.000}                       \\ \hline
\end{tabular}

\caption{\re{Normality test for \rsm\ values in Figure~\ref{fig: rsm improvement}. }} 
\label{tab: normality test fig 21}
\end{table}

Afterward, we tested the dependency between the data populations using the Spearman correlation test (as the normality test has been rejected for all populations). Table~\ref{tab: dependency test fig 21} shows the result of these tests.

\begin{table}[h]
\center
\begin{tabular}{c|c|c|}
\cline{2-3}
\multicolumn{1}{l|}{}                                       & Approach          & \begin{tabular}[c]{@{}c@{}}p-value \\ Spearman correlation test\end{tabular} \\ \hhline{-==}
\multicolumn{1}{|c|}{\multirow{4}{*}{no drift}}             & (ML2ASR, LSA)            & \reject{0.000}                       \\ \cline{2-3} 
\multicolumn{1}{|c|}{}                                      & (ML2ASR, LSA with operator)               & \accept{0.161}                         \\ \cline{2-3} 
\multicolumn{1}{|c|}{}                                      & (LSA, LSA with operator) & \accept{0.141}                       \\ \hline
\end{tabular}

\caption{\re{Dependecy test for \rsm\ values in Figure~\ref{fig: rsm improvement}. }} 
\label{tab: dependency test fig 21}
\end{table}


Based on the normality and dependency test results, we tested pairs of equality in the hypothesis (corrected by the Bonferroni method), as their results are represented in Table~\ref{tab: hypothesis 1 figure 21}.


\begin{table}[h]
\center
\begin{adjustbox}{max width=\textwidth}
\begin{tabular}{|c|c|c|}
\hline
 Hypothesis & p-value & Test method \\ \hhline{===}
$\mu_{n, r,\text{ML2ASR}} = \mu_{n, r,\text{LSA}}$& \accept{1.000} & Mann-Whitney U  \\ \hline
$\mu_{n, r,\text{ML2ASR}} = \mu_{n, r,\text{LSA\_with\_op}}$& \reject{0.022} &  Wilcoxon signed-rank\\ \hline
$\mu_{n, r,\text{LSA}} = \mu_{n, r,\text{LSA\_with\_op}}$& \reject{0.012} & Wilcoxon signed-rank\\ \hline
\end{tabular}
\end{adjustbox}
\caption{\re{Test results for this null hypothesis: ``The three approaches perform equally well with regards to \rsm\ without drift of adaptation spaces''}}
\label{tab: hypothesis 1 figure 21}
\end{table}


\subsection{Utility for All Preference Orders of Stakeholders Split For Classes Appearance Orders (Figure~\ref{fig: utility total for class appearances})}
\label{sec: appendix fig 22}
Figure~\ref{fig: utility total for class appearances} illustrates the utility for all preference orders of stakeholders split for classes appearance orders.
We have the following set of null hypotheses and their alternatives related to this figure that $\mu_{i,j,k}$ represents the mean of distribution for the utility of an approach in a subfigure, denoted by $i$ in $\mu_{i,j,k}$ that its possible values can be $a,b,c,d,e,$ and $f$. $j$ in $\mu_{i,j,k}$ indicates the metric value which is $u$ here. Finally, $k$ in $\mu_{i,j,k}$  indicates the approach that has been used.

\begin{itemize}
    \item For scenario (a), the difference in mean utility between the evolving classifier with LSA and operator feedback, and the pre-defined classifier with ML2ASR is zero or (alternatively) greater than zero:

\begin{align*}
        H_0^{(1)}: & \mu_{a, u,\text{LSA with operator}} = \mu_{a, u,\text{ML2ASR}} \\
        H_1^{(1)}: & \mu_{a, u,\text{LSA with operator}} > \mu_{a, u,\text{ML2ASR}}
\end{align*}

 \item For scenario (a), the difference in mean utility between the evolving classifier with LSA and operator feedback, and the pre-defined classifier with LSA is zero or (alternatively) greater than zero:

\begin{align*}
        H_0^{(2)}: & \mu_{a, u,\text{LSA with operator}} = \mu_{a, u,\text{LSA}} \\
        H_1^{(2)}: & \mu_{a, u,\text{LSA with operator}} > \mu_{a, u,\text{LSA}}
\end{align*}


\item For scenario (a), the difference in mean utility between the predefined classifier with ML2ASR and  he predefined classifier with LSA
with no operator feedback is zero:

\begin{align*}
        H_0^{(3)}: & \mu_{a, u,\text{ML2ASR}} = \mu_{a, u,\text{LSA}} 
\end{align*}

\item For scenario (e), the difference in mean utility between the evolving classifier with LSA and operator feedback, and ML2ASR is zero or (alternatively) greater than zero:

\begin{align*}
        H_0^{(4)}: & \mu_{e, u,\text{LSA with operator}} = \mu_{e, u,\text{ML2ASR}} \\
        H_1^{(4)}: & \mu_{e, u,\text{LSA with operator}} > \mu_{e, u,\text{ML2ASR}}
\end{align*}

 \item For scenario (e), the difference in mean utility between the evolving classifier with LSA and operator feedback, and the pre-defined classifier with LSA is zero or (alternatively) greater than zero:

\begin{align*}
        H_0^{(5)}: & \mu_{e, u,\text{LSA with operator}} = \mu_{e, u,\text{LSA}} \\
        H_1^{(5)}: & \mu_{e, u,\text{LSA with operator}} > \mu_{e, u,\text{LSA}}
\end{align*}

\item For scenario (b), the difference in mean utility between the evolving classifier with LSA and operator feedback and other approaches is zero:

        \begin{align*}
            H_0^{(6)}: & \mu_{b, u,\text{LSA\_with\_op}} = \mu_{b, u,\text{baseline}}, 
                   \mu_{b, u,\text{LSA\_with\_op}} = \mu_{b, u,\text{ML2ASR}},
                   \mu_{b, u,\text{LSA\_with\_op}} = \mu_{b, u,\text{LSA}}
        \end{align*}

\item For scenario (c), the difference in mean utility between the evolving classifier with LSA and operator feedback and other approaches is zero:

        \begin{align*}
            H_0^{(7)}: & \mu_{c, u,\text{LSA\_with\_op}} = \mu_{c, u,\text{baseline}}, 
                   \mu_{c, u,\text{LSA\_with\_op}} = \mu_{c, u,\text{ML2ASR}},
                   \mu_{c, u,\text{LSA\_with\_op}} = \mu_{c, u,\text{LSA}}
        \end{align*}

\item For scenario (d), the difference in mean utility between the evolving classifier with LSA and operator feedback and other approaches is zero:

        \begin{align*}
            H_0^{(8)}: & \mu_{d, u,\text{LSA\_with\_op}} = \mu_{d, u,\text{baseline}}, 
                   \mu_{d, u,\text{LSA\_with\_op}} = \mu_{d, u,\text{ML2ASR}},
                   \mu_{d, u,\text{LSA\_with\_op}} = \mu_{d, u,\text{LSA}}
        \end{align*}

\item For scenario (f), the difference in mean utility between the evolving classifier with LSA and operator feedback and other approaches is zero:

        \begin{align*}
            H_0^{(9)}: & \mu_{f, u,\text{ML2ASR}} = \mu_{f, u,\text{LSA}}, 
                   \mu_{f, u,\text{LSA\_with\_op}} = \mu_{f, u,\text{ML2ASR}},
                   \mu_{f, u,\text{LSA\_with\_op}} = \mu_{f, u,\text{LSA}}
        \end{align*}

\item For scenario (f), the difference in mean utility between the baseline and other approaches is zero:

        \begin{align*}
            H_0^{(10)}: &  \mu_{f, u,\text{baseline}} = \mu_{f, u,\text{ML2ASR}},
                   \mu_{f, u,\text{baseline}} = \mu_{f, u,\text{LSA}}, 
                   \mu_{f, u,\text{baseline}} = \mu_{f, u,\text{LSA\_with\_op}}
        \end{align*}

% \item For scenario (e), the difference in mean utility between LSA and ML2ASR is zero:

%         \begin{align*}
%             H_0^{(11)}: &  \mu_{e, u,\text{LSA}} = \mu_{e, u,\text{ML2ASR}}
%         \end{align*}

\end{itemize}

Like previous cases, we ran multiple tests for the normality of distributions by the Anderson-Darling method. Table~\ref{tab: normality test fig 22} shows the results and indicates all tests have been rejected (with a significance level of 0.05).


\begin{table}[h]
\center
\begin{adjustbox}{max width=\textwidth}
\begin{tabular}{|c|c|c|c|c|c|c|}
\hline
 Approach & \begin{tabular}[c]{@{}c@{}}p-value (a)\end{tabular}
          & \begin{tabular}[c]{@{}c@{}}p-value (b)\end{tabular}
          & \begin{tabular}[c]{@{}c@{}}p-value (c)\end{tabular}
          & \begin{tabular}[c]{@{}c@{}}p-value (d)\end{tabular}
          & \begin{tabular}[c]{@{}c@{}}p-value (e)\end{tabular}
          & \begin{tabular}[c]{@{}c@{}}p-value (f)\end{tabular}\\ \hhline{=======}
Baseline &  \reject{0.000} & \reject{0.000} & \reject{0.000} & \reject{0.000} & \reject{0.000} & \reject{0.000}\\ \hline
ML2ASR &   \reject{0.000} & \reject{0.000} & \reject{0.000} & \reject{0.000} & \reject{0.000} & \reject{0.000}\\ \hline
LSA &   \reject{0.000} & \reject{0.000} & \reject{0.000} & \reject{0.000} & \reject{0.000} & \reject{0.000}\\ \hline
LSA with operator &   \reject{0.000} & \reject{0.000} & \reject{0.000} & \reject{0.000} & \reject{0.000} & \reject{0.000}\\ \hline
\end{tabular}
\end{adjustbox}
\caption{\re{Normality tests for distributions in subfigures of Figure~\ref{fig: utility total for class appearances}, by Anderson-Darling test method }}
\label{tab: normality test fig 22}
\end{table}

Based on rejection of all normality tests, we used the Spearman correlation method to test the dependency (as in previous cases). Test results in Table~\ref{tab: dependency test fig 22} indicate dependency tests for all pairs were rejected with a significance level of 0.05.

\begin{table}[h]
\center
\begin{adjustbox}{max width=\textwidth}
\begin{tabular}{|c|c|c|c|c|c|c|}
\hline
 Approach & \begin{tabular}[c]{@{}c@{}}p-value (a)\end{tabular}
          & \begin{tabular}[c]{@{}c@{}}p-value (b)\end{tabular}
          & \begin{tabular}[c]{@{}c@{}}p-value (c)\end{tabular}
          & \begin{tabular}[c]{@{}c@{}}p-value (d)\end{tabular}
          & \begin{tabular}[c]{@{}c@{}}p-value (e)\end{tabular}
          & \begin{tabular}[c]{@{}c@{}}p-value (f)\end{tabular}\\ \hhline{=======}
(Baseline, ML2ASR) &  \reject{0.000} & \reject{0.000} & \reject{0.000} & \reject{0.000} & \reject{0.000} & \reject{0.000}\\ \hline
(Baseline, LSA) &   \reject{0.000} & \reject{0.000} & \reject{0.000} & \reject{0.000} & \reject{0.000} & \reject{0.000}\\ \hline
(Baseline, LSA with operator) &   \reject{0.000} & \reject{0.000} & \reject{0.000} & \reject{0.000} & \reject{0.000} & \reject{0.000}\\ \hline
(ML2ASR, LSA) &   \reject{0.000} & \reject{0.000} & \reject{0.000} & \reject{0.000} & \reject{0.000} & \reject{0.000}\\ \hline
(ML2ASR, LSA with operator) &   \reject{0.000} & \reject{0.000} & \reject{0.000} & \reject{0.000} & \reject{0.000} & \reject{0.000}\\ \hline
(LSA, LSA with operator) &   \reject{0.000} & \reject{0.000} & \reject{0.000} & \reject{0.000} & \reject{0.000} & \reject{0.000}\\ \hline
\end{tabular}
\end{adjustbox}
\caption{\re{Dependency tests for distributions in subfigures of Figure~\ref{fig: utility total for class appearances}, by Spearman correlation test method}}
\label{tab: dependency test fig 22}
\end{table}

We tested the hypotheses with an appropriate test method based on the normality and dependency test results; see Table~\ref{tab: hypotheses test fig 22}.

\begin{table}[h]
\center
\begin{adjustbox}{max width=\textwidth}
\begin{tabular}{|c|c|c|c|}
\hline
\multicolumn{2}{|c|}{Hypothesis}  & p-value & Test method \\ \hhline{====}
\multicolumn{2}{|l|}{\begin{tabular}[c]{@{}c@{}}
$H_0^{(1)}: \mu_{a, u,\text{LSA with operator}} = \mu_{a,u,\text{ML2ASR}}$ \\ 
        $H_1^{(1)}: \mu_{a, u,\text{LSA with operator}} > \mu_{a, u,\text{ML2ASR}}$\end{tabular}}& \reject{0.000} & Mann-Whitney U  \\ \hhline{====}
\multicolumn{2}{|l|}{\begin{tabular}[c]{@{}c@{}}
$H_0^{(2)}: \mu_{a, u,\text{LSA with operator}} = \mu_{a,u,\text{LSA}}$ \\
        $H_1^{(2)}: \mu_{a, u,\text{LSA with operator}} > \mu_{a, u,\text{LSA}}$\end{tabular}}& \reject{0.000} & Mann-Whitney U  \\ \hhline{====}
\multicolumn{2}{|l|}{$H_0^{(3)}: \mu_{a, u,\text{ML2ASR}} = \mu_{a, u,\text{LSA with operator}}$}& \accept{0.495} & Mann-Whitney U  \\ \hhline{====}

\multicolumn{2}{|l|}{\begin{tabular}[c]{@{}c@{}}
$H_0^{(4)}: \mu_{e, u,\text{LSA with operator}} = \mu_{e,u,\text{ML2ASR}}$ \\
        $H_1^{(4)}: \mu_{e, u,\text{LSA with operator}} > \mu_{e, u,\text{ML2ASR}}$\end{tabular}}& \reject{0.000} & Mann-Whitney U  \\ \hhline{====}
\multicolumn{2}{|l|}{\begin{tabular}[c]{@{}c@{}}
$H_0^{(5)}: \mu_{e, u,\text{LSA with operator}} = \mu_{e,u,\text{LSA}}$ \\
        $H_1^{(5)}: \mu_{e, u,\text{LSA with operator}} > \mu_{e, u,\text{LSA}}$\end{tabular}}& \reject{0.000} & Mann-Whitney U  \\ \hhline{====}
\multicolumn{1}{|l|}{\multirow{3}{*}{$H_0^{(6)}$}} & $\mu_{b, u,\text{LSA\_with\_op}} = \mu_{b, u,\text{baseline}}$& \accept{0.249} &  Mann-Whitney U \\ \cline{2-4} 
\multicolumn{1}{|l|}{} & $\mu_{b, u,\text{LSA\_with\_op}} = \mu_{b, u,\text{ML2ASR}}$& \reject{0.000} &  Mann-Whitney U \\ \cline{2-4} 
\multicolumn{1}{|l|}{} &  $\mu_{b, u,\text{LSA\_with\_op}} = \mu_{b, u,\text{LSA}}$& \reject{0.000} &  Mann-Whitney U
\\ \hhline{====}
\multicolumn{1}{|l|}{\multirow{3}{*}{$H_0^{(7)}$}} & 
$\mu_{c, u,\text{LSA\_with\_op}} = \mu_{c, u,\text{baseline}}$& \accept{0.753} &  Mann-Whitney U\\ \cline{2-4}
\multicolumn{1}{|l|}{} &$\mu_{c, u,\text{LSA\_with\_op}} = \mu_{c, u,\text{ML2ASR}}$& \accept{0.759} &  Mann-Whitney U\\ \cline{2-4}
\multicolumn{1}{|l|}{} &$\mu_{c, u,\text{LSA\_with\_op}} = \mu_{c, u,\text{LSA}}$& \accept{0.490} &  Mann-Whitney U\\ \hhline{====}
\multicolumn{1}{|l|}{\multirow{3}{*}{$H_0^{(8)}$}} & 
$\mu_{d, u,\text{LSA\_with\_op}} = \mu_{d, u,\text{baseline}}$& \accept{0.847} &  Mann-Whitney U\\ \cline{2-4}
\multicolumn{1}{|l|}{} &$\mu_{d, u,\text{LSA\_with\_op}} = \mu_{d, u,\text{ML2ASR}}$& \accept{1.000} &  Mann-Whitney U\\ \cline{2-4}
\multicolumn{1}{|l|}{} &$\mu_{d, u,\text{LSA\_with\_op}} = \mu_{d, u,\text{LSA}}$& \accept{1.000} &  Mann-Whitney U\\ \hhline{====}
\multicolumn{1}{|l|}{\multirow{3}{*}{$H_0^{(9)}$}} &
$\mu_{f, u,\text{ML2ASR}} = \mu_{f, u,\text{LSA}}$& \accept{0.919} &  Mann-Whitney U\\ \cline{2-4}
\multicolumn{1}{|l|}{} & $\mu_{f, u,\text{LSA\_with\_op}} = \mu_{f, u,\text{ML2ASR}}$& \accept{1.000} &  Mann-Whitney U\\ \cline{2-4}
\multicolumn{1}{|l|}{} & $\mu_{f, u,\text{LSA\_with\_op}} = \mu_{f, u,\text{LSA}}$& \accept{0.573} &  Mann-Whitney U\\ \hhline{====}
\multicolumn{1}{|l|}{\multirow{3}{*}{$H_0^{(10)}$}} &
$\mu_{f, u,\text{baseline}} = \mu_{f, u,\text{ML2ASR}}$& \reject{0.006} &  Mann-Whitney U\\ \cline{2-4}
\multicolumn{1}{|l|}{} & $\mu_{f, u,\text{baseline}} = \mu_{f, u,\text{LSA}}$& \reject{0.002} &  Mann-Whitney U\\ \cline{2-4}
\multicolumn{1}{|l|}{} & $\mu_{f, u,\text{baseline}} = \mu_{f, u,\text{LSA\_with\_op}}$& \reject{0.008} &  Mann-Whitney U
% \\ \hhline{====}
% \multicolumn{2}{|l|}{$H_0^{(11)}: \mu_{e, u,\text{LSA}} = \mu_{e, u,\text{ML2ASR}}$}& \accept{0.050} & Mann-Whitney U  
\\ \hline
\end{tabular}
\end{adjustbox}
\caption{\re{Test results for all mentioned hypotheses for Figure~\ref{fig: utility total for class appearances}, separated by double horizontal lines.}}
\label{tab: hypotheses test fig 22}
\end{table}


%%%%%%%%%%%%%%%%%%%%%%%%%%%%%%%%%%%% RSM %%%%%%%%%%%%%%%%%%%%%%%%%%%%%%%%%%%%
\subsection{\rsm\ for All Preference Orders of Stakeholders Split for Classes Appearance Order (Figure~\ref{fig: rsm total for class appearances})}
\label{sec: appendix fig 23}
Figure~\ref{fig: rsm total for class appearances} illustrates the utility for all preference orders of stakeholders split for classes appearance orders.
We have the following set of null hypotheses and their alternatives related to this figure, such that $\mu_{i,r,k}$ represents the mean of distribution for the utility of an approach in a subfigure denoted by $i$ in $\mu_{i,r,k}$. The possible values of $i$ can be $a,b,c,d,e,$ and $f$. $r$ in $\mu_{i,j,k}$ indicates the metric value which is \rsm\ here. Finally, $k$ in $\mu_{i,j,k}$  indicates the approach that has been used.
Also, for the sake of brevity, we used $n$ in $H_0^{(n)}$ and $H_1^{(n)}$ to show the identifier of the corresponding null hypothesis and its alternative. This identifier helps us to refer to these hypotheses afterward.

\begin{itemize}
    \item For scenario (a), the difference in mean \rsm\ between the evolving classifier with LSA and operator feedback, and the pre-defined classifier with ML2ASR is zero or (alternatively) less than zero:

\begin{align*}
        H_0^{(1)}: & \mu_{a, r,\text{LSA with operator}} = \mu_{a, r,\text{ML2ASR}} \\
        H_1^{(1)}: & \mu_{a, r,\text{LSA with operator}} < \mu_{a, r,\text{ML2ASR}}
\end{align*}

 \item For scenario (a), the difference in mean \rsm\ between the evolving classifier with LSA and operator feedback, and the pre-defined classifier with LSA is zero or (alternatively) less than zero:

\begin{align*}
        H_0^{(2)}: & \mu_{a, r,\text{LSA with operator}} = \mu_{a, r,\text{LSA}} \\
        H_1^{(2)}: & \mu_{a, r,\text{LSA with operator}} < \mu_{a, r,\text{LSA}}
\end{align*}

 \item For scenario (a), the difference in mean \rsm\ between the predefined classifier with LSA (without operator feedback) and ML2ASR is zero:

\begin{align*}
        H_0^{(3)}: & \mu_{a, r,\text{LSA}} = \mu_{a, r,\text{ML2ASR}}
\end{align*}

\item For scenario (b), the difference in mean \rsm\ between the evolving classifier with LSA and operator feedback and other approaches is zero:

        \begin{align*}
            H_0^{(4)}: & 
                   \mu_{b, r,\text{LSA\_with\_op}} = \mu_{b, r,\text{ML2ASR}},
                   \mu_{b, r,\text{LSA\_with\_op}} = \mu_{b, r,\text{LSA}}
        \end{align*}

\item For scenario (c), the difference in mean \rsm\ between the evolving classifier with LSA and operator feedback and other approaches is zero:

        \begin{align*}
            H_0^{(5)}: & 
                   \mu_{c, r,\text{LSA\_with\_op}} = \mu_{c, r,\text{ML2ASR}},
                   \mu_{c, r,\text{LSA\_with\_op}} = \mu_{c, r,\text{LSA}}
        \end{align*}

\item For scenario (d), the difference in mean \rsm\ between the evolving classifier with LSA and operator feedback and other approaches is zero:

        \begin{align*}
            H_0^{(6)}: & 
                   \mu_{d, r,\text{LSA\_with\_op}} = \mu_{d, r,\text{ML2ASR}},
                   \mu_{d, r,\text{LSA\_with\_op}} = \mu_{d, r,\text{LSA}}
        \end{align*}

\item For scenario (e), the difference in mean \rsm\ between predefined classifier with LSA (without operator feedback) and ML2ASR is zero:

        \begin{align*}
            H_0^{(7)}: &
                   \mu_{e, r,\text{LSA}} = \mu_{e, r,\text{ML2ASR}}
        \end{align*}

\item For scenario (f), the difference in mean \rsm\ between the evolving classifier with LSA and operator feedback and other approaches is zero:

        \begin{align*}
            H_0^{(8)}: &
                   \mu_{f, r,\text{LSA\_with\_op}} = \mu_{f, r,\text{ML2ASR}},
                   \mu_{f, r,\text{LSA\_with\_op}} = \mu_{f, r,\text{LSA}}
        \end{align*}
\end{itemize}


Like previous cases, we ran multiple tests for the normality of distributions by the Anderson-Darling method. Table~\ref{tab: hypotheses test fig 23} shows the results and indicates all tests have been rejected (with a significance level of 0.05).


\begin{table}[h]
\center
\begin{adjustbox}{max width=\textwidth}
\begin{tabular}{|c|c|c|c|c|c|c|}
\hline
 Approach & \begin{tabular}[c]{@{}c@{}}p-value (a)\end{tabular}
          & \begin{tabular}[c]{@{}c@{}}p-value (b)\end{tabular}
          & \begin{tabular}[c]{@{}c@{}}p-value (c)\end{tabular}
          & \begin{tabular}[c]{@{}c@{}}p-value (d)\end{tabular}
          & \begin{tabular}[c]{@{}c@{}}p-value (e)\end{tabular}
          & \begin{tabular}[c]{@{}c@{}}p-value (f)\end{tabular}\\ \hhline{=======}
ML2ASR &   \reject{0.001} & \reject{0.001} & \reject{0.000} & \reject{0.000} & \reject{0.028} & \reject{0.000}\\ \hline
LSA &   \reject{0.009} & \reject{0.000} & \reject{0.000} & \reject{0.000} & \reject{0.043} & \reject{0.000}\\ \hline
LSA with operator &   \reject{0.000} & \reject{0.003} & \reject{0.000} & \reject{0.000} & \reject{0.000} & \reject{0.000}\\ \hline
\end{tabular}
\end{adjustbox}
\caption{\re{Normality tests for distributions in subfigures of Figure~\ref{fig: rsm total for class appearances}, by Anderson-Darling test method }}
\label{tab: normality test fig 23}
\end{table}


Based on rejection of all normality tests, we used the Spearman correlation method to test the dependency (as in previous cases). Test results in Table~\ref{tab: dependency test fig 23} indicate dependency tests for all pairs were rejected with a significance level of 0.05.
\begin{table}[h]
\center
\begin{adjustbox}{max width=\textwidth}
\begin{tabular}{|c|c|c|c|c|c|c|}
\hline
 Approach & \begin{tabular}[c]{@{}c@{}}p-value (a)\end{tabular}
          & \begin{tabular}[c]{@{}c@{}}p-value (b)\end{tabular}
          & \begin{tabular}[c]{@{}c@{}}p-value (c)\end{tabular}
          & \begin{tabular}[c]{@{}c@{}}p-value (d)\end{tabular}
          & \begin{tabular}[c]{@{}c@{}}p-value (e)\end{tabular}
          & \begin{tabular}[c]{@{}c@{}}p-value (f)\end{tabular}\\ \hhline{=======}
(ML2ASR, LSA) &   \reject{0.000} & \reject{0.000} & \reject{0.000} & \reject{0.000} & \reject{0.000} & \reject{0.000}\\ \hline
(ML2ASR, LSA with operator) &   \reject{0.009} & \reject{0.000} & \reject{0.000} & \reject{0.000} & \reject{0.000} & \reject{0.000}\\ \hline
(LSA, LSA with operator) &   \reject{0.027} & \reject{0.000} & \reject{0.000} & \reject{0.000} & \reject{0.000} & \reject{0.000}\\ \hline
\end{tabular}
\end{adjustbox}
\caption{\re{Dependency tests for distributions in subfigures of Figure~\ref{fig: rsm total for class appearances}, by Spearman correlation test method}}
\label{tab: dependency test fig 23}
\end{table}

We tested the hypotheses with an appropriate test method based on the normality and dependency test results; see Table~\ref{tab: hypotheses test fig 23}.

% \begin{table}[h]
% \center
% \begin{adjustbox}{max width=\textwidth}
% \begin{tabular}{|c|c|c|}
% \hline
%  Hypothesis & p-value & Test method \\ \hhline{===}
% \begin{tabular}[c]{@{}c@{}}
% $H_0^{(1)}: \mu_{a, r,\text{LSA with operator}} = \mu_{a,r,\text{ML2ASR}}$ \\
%         $H_1^{(1)}: \mu_{a, r,\text{LSA with operator}} < \mu_{a, r,\text{ML2ASR}}$\end{tabular}& \reject{0.000} & Mann-Whitney U  \\ \hhline{===}
% \begin{tabular}[c]{@{}c@{}}
% $H_0^{(2)}: \mu_{a, r,\text{LSA with operator}} = \mu_{a,r,\text{LSA}}$ \\
%         $H_1^{(2)}: \mu_{a, r,\text{LSA with operator}} < \mu_{a, r,\text{LSA}}$\end{tabular}& \reject{0.000} & Mann-Whitney U  \\ \hhline{===}
% $\mu_{b, r,\text{LSA\_with\_op}} = \mu_{b, r,\text{ML2ASR}}$& \reject{0.048} &  Mann-Whitney U\\ \hline
% $\mu_{b, r,\text{LSA\_with\_op}} = \mu_{b, r,\text{LSA}}$& \reject{0.040} &  Mann-Whitney U\\ \hhline{===}
% $\mu_{c, r,\text{LSA\_with\_op}} = \mu_{c, r,\text{ML2ASR}}$& \reject{0.018} &  Mann-Whitney U\\ \hline
% $\mu_{c, r,\text{LSA\_with\_op}} = \mu_{c, r,\text{LSA}}$& \reject{0.019} &  Mann-Whitney U\\ \hhline{===}
% $\mu_{d, r,\text{LSA\_with\_op}} = \mu_{d, r,\text{ML2ASR}}$& \reject{0.025} &  Mann-Whitney U\\ \hline
% $\mu_{d, r,\text{LSA\_with\_op}} = \mu_{d, r,\text{LSA}}$& \reject{0.027} &  Mann-Whitney U\\ \hhline{===}

% $\mu_{f, r,\text{LSA\_with\_op}} = \mu_{f, r,\text{ML2ASR}}$& \accept{0.683} &  Mann-Whitney U\\ \hline
% $\mu_{f, r,\text{LSA\_with\_op}} = \mu_{f, r,\text{LSA}}$& \accept{0.894} &  Mann-Whitney U\\ \hline
% \end{tabular}
% \end{adjustbox}
% \caption{\re{Test results for all mentioned hypotheses for Figure~\ref{fig: utility total for class appearnces}, separated by double horizontal lines.}}
% \end{table}

%%%%%%%%%%%%%%%%%%%%%%%%%%%%%%%%%% New TABLE %%%%%%%%%%%%%%%%%%%


\begin{table}[h]
\center
\begin{adjustbox}{max width=\textwidth}
\begin{tabular}{|c|c|c|c|}
\hline
\multicolumn{2}{|c|}{Hypothesis}  & p-value & Test method \\ \hhline{====}
\multicolumn{2}{|l|}{\begin{tabular}[c]{@{}c@{}}
$H_0^{(1)}: \mu_{a, r,\text{LSA with operator}} = \mu_{a,r,\text{ML2ASR}}$ \\
        $H_1^{(1)}: \mu_{a, r,\text{LSA with operator}} < \mu_{a, r,\text{ML2ASR}}$\end{tabular}}& \reject{0.000} & Mann-Whitney U  \\ \hhline{====}
\multicolumn{2}{|l|}{\begin{tabular}[c]{@{}c@{}}
$H_0^{(2)}: \mu_{a, r,\text{LSA with operator}} = \mu_{a,r,\text{LSA}}$ \\
        $H_1^{(2)}: \mu_{a, r,\text{LSA with operator}} < \mu_{a, r,\text{LSA}}$\end{tabular}}& \reject{0.000} & Mann-Whitney U  \\ \hhline{====}
\multicolumn{2}{|l|}{
$H_0^{(3)}: \mu_{a, r,\text{LSA}} = \mu_{a,r,\text{ML2ASR}}$}& \accept{0.494} & Mann-Whitney U  \\ \hhline{====}
\multicolumn{1}{|l|}{\multirow{2}{*}{$H_0^{(4)}$}} & $\mu_{b, r,\text{LSA\_with\_op}} = \mu_{b, r,\text{ML2ASR}}$& \reject{0.048} &  Mann-Whitney U \\ \cline{2-4} 
\multicolumn{1}{|l|}{} & $\mu_{b, r,\text{LSA\_with\_op}} = \mu_{b, r,\text{LSA}}$& \reject{0.040} &  Mann-Whitney U
\\ \hhline{====}
\multicolumn{1}{|l|}{\multirow{2}{*}{$H_0^{(5)}$}} & $\mu_{c, r,\text{LSA\_with\_op}} = \mu_{c, r,\text{ML2ASR}}$& \reject{0.018} &  Mann-Whitney U \\ \cline{2-4} 
\multicolumn{1}{|l|}{} & $\mu_{c, r,\text{LSA\_with\_op}} = \mu_{c, r,\text{LSA}}$& \reject{0.019} &  Mann-Whitney U
\\ \hhline{====}
\multicolumn{1}{|l|}{\multirow{2}{*}{$H_0^{(6)}$}} & $\mu_{d, r,\text{LSA\_with\_op}} = \mu_{d, r,\text{ML2ASR}}$& \reject{0.025} &  Mann-Whitney U \\ \cline{2-4} 
\multicolumn{1}{|l|}{} & $\mu_{d, r,\text{LSA\_with\_op}} = \mu_{d, r,\text{LSA}}$& \reject{0.027} &  Mann-Whitney U
\\ \hhline{====}

\multicolumn{2}{|l|}{
$H_0^{(7)}: \mu_{e, r,\text{LSA}} = \mu_{e,r,\text{ML2ASR}}$}& \accept{0.469} & Mann-Whitney U  \\ \hhline{====}

\multicolumn{1}{|l|}{\multirow{2}{*}{$H_0^{(8)}$}} & $\mu_{f, r,\text{LSA\_with\_op}} = \mu_{f, r,\text{ML2ASR}}$& \accept{0.683} &  Mann-Whitney U \\ \cline{2-4} 
\multicolumn{1}{|l|}{} & $\mu_{f, r,\text{LSA\_with\_op}} = \mu_{f, r,\text{LSA}}$& \accept{0.894} &  Mann-Whitney U
\\ \hline

\end{tabular}
\end{adjustbox}
\caption{\re{Test results for all mentioned hypotheses for Figure~\ref{fig: rsm total for class appearances}, separated by double horizontal lines.}}
\label{tab: hypotheses test fig 23}
\end{table}





\subsection{Utility for All Class Appearance Order Scenarios Split for Preference Order of Stakeholders (Figure~\ref{fig: utility total})}
\label{sec: appendix fig 24}
Figure~\ref{fig: utility total} illustrates the utility for all class appearance order scenarios split for preference order of stakeholders.
We have the following set of null hypotheses and their alternatives related to this figure:

\begin{itemize}
    \item For scenario (a), the difference in mean utility between the evolving classifier with LSA and operator feedback, and the pre-defined classifier with ML2ASR is zero or (alternatively) greater than zero:

\begin{align*}
        H_0^{(1)}: & \mu_{a, u,\text{LSA with operator}} = \mu_{a, u,\text{ML2ASR}} \\
        H_1^{(1)}: & \mu_{a, u,\text{LSA with operator}} > \mu_{a, u,\text{ML2ASR}}
\end{align*}

 \item For scenario (a), the difference in mean utility between the evolving classifier with LSA and operator feedback, and the pre-defined classifier with LSA is zero or (alternatively) greater than zero:

\begin{align*}
        H_0^{(2)}: & \mu_{a, u,\text{LSA with operator}} = \mu_{a, u,\text{LSA}} \\
        H_1^{(2)}: & \mu_{a, u,\text{LSA with operator}} > \mu_{a, u,\text{LSA}}
\end{align*}

 \item For scenario (a), the difference in mean utility between the evolving classifier with LSA and operator feedback, and the baseline is zero:

\begin{align*}
        H_0^{(3)}: & \mu_{a, u,\text{LSA with operator}} = \mu_{a, u,\text{baseline}} 
\end{align*}

 \item For scenario (a), the difference in mean utility between the pre-defined classifier with LSA (without feedback) and ML2ASR is zero:

\begin{align*}
        H_0^{(4)}: & \mu_{a, u,\text{LSA}} = \mu_{a, u,\text{ML2ASR}} 
\end{align*}

 \item For scenario (b), the difference in mean utility between the evolving classifier with LSA and operator feedback, and the pre-defined classifier with ML2ASR is zero or (alternatively) greater than zero:

\begin{align*}
        H_0^{(5)}: & \mu_{b, u,\text{LSA with operator}} = \mu_{b, u,\text{ML2ASR}} \\
        H_1^{(5)}: & \mu_{b, u,\text{LSA with operator}} > \mu_{b, u,\text{ML2ASR}}
\end{align*}

 \item For scenario (b), the difference in mean utility between the evolving classifier with LSA and operator feedback, and the pre-defined classifier with LSA is zero or (alternatively) greater than zero:

\begin{align*}
        H_0^{(6)}: & \mu_{b, u,\text{LSA with operator}} = \mu_{b, u,\text{LSA}} \\
        H_1^{(6)}: & \mu_{b, u,\text{LSA with operator}} > \mu_{b, u,\text{LSA}}
\end{align*}

 \item For scenario (b), the difference in mean utility between the evolving classifier with LSA and operator feedback, and the baseline is zero:

\begin{align*}
        H_0^{(7)}: & \mu_{b, u,\text{LSA with operator}} = \mu_{b, u,\text{baseline}} 
\end{align*}

 \item For scenario (b), the difference in mean utility between the pre-defined classifier with LSA (without operator feedback) and ML2ASR is zero:

\begin{align*}
        H_0^{(8)}: & \mu_{b, u,\text{LSA}} = \mu_{b, u,\text{ML2ASR}} 
\end{align*}

\end{itemize}

Like previous cases, we ran multiple tests for the normality of distributions by the Anderson-Darling method. Table~\ref{tab: normality test fig 24} shows the results and indicates all tests have been rejected (with a significance level of 0.05).


\begin{table}[h]
\center
\begin{adjustbox}{max width=\textwidth}
\begin{tabular}{|c|c|c|}
\hline
 Approach & \begin{tabular}[c]{@{}c@{}}p-value (a)\end{tabular}
          & \begin{tabular}[c]{@{}c@{}}p-value (b)\end{tabular} \\ \hhline{===}
Baseline &  \reject{0.000} & \reject{0.000} \\ \hline
ML2ASR &   \reject{0.000} & \reject{0.000} \\ \hline
LSA &   \reject{0.000} & \reject{0.000} \\ \hline
LSA with operator &   \reject{0.000} & \reject{0.000} \\ \hline
\end{tabular}
\end{adjustbox}
\caption{\re{Normality tests for distributions in subfigures of Figure~\ref{fig: utility total}, by Anderson-Darling test method }}
\label{tab: normality test fig 24}
\end{table}

Based on rejection of all normality tests, we used the Spearman correlation method to test the dependency (as in previous cases). Test results in Table~\ref{tab: dependency test fig 24} indicate dependency tests for all pairs were rejected with a significance level of 0.05.

\begin{table}[h]
\center
\begin{adjustbox}{max width=\textwidth}
\begin{tabular}{|c|c|c|}
\hline
 Approach & \begin{tabular}[c]{@{}c@{}}p-value (a)\end{tabular}
          & \begin{tabular}[c]{@{}c@{}}p-value (b)\end{tabular}\\ \hhline{===}
(Baseline, ML2ASR) &  \reject{0.000} & \reject{0.000} \\ \hline
(Baseline, LSA) &   \reject{0.000} & \reject{0.000} \\ \hline
(Baseline, LSA with operator) &   \accept{0.107} & \reject{0.000} \\ \hline
(ML2ASR, LSA) &   \reject{0.000} & \reject{0.000} \\ \hline
(ML2ASR, LSA with operator) &   \accept{0.075} & \reject{0.000}\\ \hline
(LSA, LSA with operator) &   \accept{0.053} & \reject{0.001} \\ \hline
\end{tabular}
\end{adjustbox}
\caption{\re{Dependency tests for distributions in subfigures of Figure~\ref{fig: utility total}, by Spearman correlation test method}}
\label{tab: dependency test fig 24}
\end{table}

We tested the hypotheses with an appropriate test method based on the normality and dependency test results; see Table~\ref{tab: hypotheses test fig 24}.

% \begin{table}[h]
% \center
% \begin{adjustbox}{max width=\textwidth}
% \begin{tabular}{|c|c|c|}
% \hline
%  Hypothesis & p-value & Test method \\ \hhline{===}
% \begin{tabular}[c]{@{}c@{}}
% $H_0: \mu_{a, u,\text{LSA with operator}} = \mu_{a,u,\text{ML2ASR}}$ \\
%         $H_1: \mu_{a, u,\text{LSA with operator}} > \mu_{a, u,\text{ML2ASR}}$\end{tabular}& \reject{0.000} & Wilcoxon signed-rank  \\ \hhline{===}
% \begin{tabular}[c]{@{}c@{}}
% $H_0: \mu_{a, u,\text{LSA with operator}} = \mu_{a,u,\text{LSA}}$ \\
%         $H_1: \mu_{a, u,\text{LSA with operator}} > \mu_{a, u,\text{LSA}}$\end{tabular}& \reject{0.000} & Wilcoxon signed-rank  \\ \hhline{===}
% \begin{tabular}[c]{@{}c@{}}
% $H_0: \mu_{a, u,\text{LSA with operator}} = \mu_{a,u,\text{baseline}}$ \end{tabular}& \accept{0.830} & Wilcoxon signed-rank  \\ \hhline{===}
% \begin{tabular}[c]{@{}c@{}}
% $H_0: \mu_{b, u,\text{LSA with operator}} = \mu_{b,u,\text{ML2ASR}}$ \\
%         $H_1: \mu_{b, u,\text{LSA with operator}} > \mu_{b, u,\text{ML2ASR}}$\end{tabular}& \reject{0.000} & Mann-Whitney U  \\ \hhline{===}

% \begin{tabular}[c]{@{}c@{}}
% $H_0: \mu_{b, u,\text{LSA with operator}} = \mu_{b,u,\text{LSA}}$ \\
%         $H_1: \mu_{b, u,\text{LSA with operator}} > \mu_{b, u,\text{LSA}}$\end{tabular}& \reject{0.000} & Mann-Whitney U  \\ \hhline{===}
% \begin{tabular}[c]{@{}c@{}}
% $H_0: \mu_{b, u,\text{LSA with operator}} = \mu_{b,u,\text{baseline}}$ \end{tabular}& \reject{0.000} & Mann-Whitney U \\ \hhline{===}

% \end{tabular}
% \end{adjustbox}
% \caption{\re{Test results for all mentioned hypotheses for Figure~\ref{fig: utility total for class appearnces}, separated by double horizontal lines.}}
% \end{table}


\begin{table}[h]
\center
\begin{adjustbox}{max width=\textwidth}
\begin{tabular}{|c|c|c|c|}
\hline
\multicolumn{2}{|c|}{Hypothesis}  & p-value & Test method \\ \hhline{====}
\multicolumn{2}{|l|}{\begin{tabular}[c]{@{}c@{}}
$H_0^{(1)}: \mu_{a, u,\text{LSA with operator}} = \mu_{a,u,\text{ML2ASR}}$ \\
        $H_1^{(1)}: \mu_{a, u,\text{LSA with operator}} > \mu_{a, u,\text{ML2ASR}}$\end{tabular}}& \reject{0.000} & Wilcoxon signed-rank  \\ \hhline{====}
\multicolumn{2}{|l|}{\begin{tabular}[c]{@{}c@{}}
$H_0^{(2)}: \mu_{a, u,\text{LSA with operator}} = \mu_{a,u,\text{LSA}}$ \\
        $H_1^{(2)}: \mu_{a, u,\text{LSA with operator}} > \mu_{a, u,\text{LSA}}$\end{tabular}}& \reject{0.000} & Wilcoxon signed-rank  \\ \hhline{====}
\multicolumn{2}{|l|}{
$H_0^{(3)}: \mu_{a, u,\text{LSA with operator}} = \mu_{a,u,\text{baseline}}$}& \accept{0.830} & Wilcoxon signed-rank  \\ \hhline{====}
\multicolumn{2}{|l|}{
$H_0^{(4)}: \mu_{a, u,\text{LSA}} = \mu_{a,u,\text{ML2ASR}}$}& \accept{0.353} & Mann-Whitney U  \\ \hhline{====}
\multicolumn{2}{|l|}{\begin{tabular}[c]{@{}c@{}}
$H_0^{(5)}: \mu_{b, u,\text{LSA with operator}} = \mu_{b,u,\text{ML2ASR}}$ \\
        $H_1^{(5)}: \mu_{b, u,\text{LSA with operator}} > \mu_{b, u,\text{ML2ASR}}$\end{tabular}}& \reject{0.000} & Mann-Whitney U  \\ \hhline{====}
\multicolumn{2}{|l|}{\begin{tabular}[c]{@{}c@{}}
$H_0^{(6)}: \mu_{b, u,\text{LSA with operator}} = \mu_{b,u,\text{LSA}}$ \\
        $H_1^{(6)}: \mu_{b, u,\text{LSA with operator}} > \mu_{b, u,\text{LSA}}$\end{tabular}}& \reject{0.000} & Mann-Whitney U  \\ \hhline{====}
\multicolumn{2}{|l|}{
$H_0^{(7)}: \mu_{b, u,\text{LSA with operator}} = \mu_{b,u,\text{baseline}}$}& \reject{0.000} & Mann-Whitney U  \\ \hhline{====}
\multicolumn{2}{|l|}{
$H_0^{(8)}: \mu_{b, u,\text{LSA}} = \mu_{b,u,\text{ML2ASR}}$}& \accept{0.394} & Mann-Whitney U  \\ \hline
\end{tabular}
\end{adjustbox}
\caption{\re{Test results for all mentioned hypotheses for Figure~\ref{fig: utility total}, separated by double horizontal lines.}}
\label{tab: hypotheses test fig 24}
\end{table}





\subsection{\rsm\ for All Class Appearance Order Scenarios Split for Preference Order of Stakeholders (Figure~\ref{fig: rsm total}) }
\label{sec: appendix fig 25}
Figure~\ref{fig: rsm total} illustrates the \rsm\ values for all class appearance order scenarios split for preference order of stakeholders.
We have the following set of null hypotheses and their alternatives related to this figure:

\begin{itemize}
    \item For scenario (a), the difference in mean \rsm\ between the evolving classifier with LSA and operator feedback, and the pre-defined classifier with ML2ASR is zero or (alternatively) less than zero:

\begin{align*}
        H_0^{(1)}: & \mu_{a, r,\text{LSA with operator}} = \mu_{a, r,\text{ML2ASR}} \\
        H_1^{(1)}: & \mu_{a, r,\text{LSA with operator}} > \mu_{a, r,\text{ML2ASR}}
\end{align*}

 \item For scenario (a), the difference in mean \rsm\ between the evolving classifier with LSA and operator feedback, and the pre-defined classifier with LSA is zero or (alternatively) less than zero:

\begin{align*}
        H_0^{(2)}: & \mu_{a, r,\text{LSA with operator}} = \mu_{a, r,\text{LSA}} \\
        H_1^{(2)}: & \mu_{a, r,\text{LSA with operator}} > \mu_{a, r,\text{LSA}}
\end{align*}

 \item For scenario (a), the difference in mean \rsm\ between the predefined classifier with LSA (without operator feedback) and ML2ASR is zero:

\begin{align*}
        H_0^{(3)}: & \mu_{a, r,\text{LSA}} = \mu_{a, r,\text{ML2ASR}}
\end{align*}


    \item For scenario (b), the difference in mean \rsm\ between the evolving classifier with LSA and operator feedback, and the pre-defined classifier with ML2ASR is zero or (alternatively) less than zero:

\begin{align*}
        H_0^{(4)}: & \mu_{b, r,\text{LSA with operator}} = \mu_{b, r,\text{ML2ASR}} \\
        H_1^{(4)}: & \mu_{b, r,\text{LSA with operator}} > \mu_{b, r,\text{ML2ASR}}
\end{align*}

 \item For scenario (b), the difference in mean \rsm\ between the evolving classifier with LSA and operator feedback, and the pre-defined classifier with LSA is zero or (alternatively) less than zero:

\begin{align*}
        H_0^{(5)}: & \mu_{b, r,\text{LSA with operator}} = \mu_{b, r,\text{LSA}} \\
        H_1^{(5)}: & \mu_{b, r,\text{LSA with operator}} > \mu_{b, r,\text{LSA}}
\end{align*}

\item For scenario (b), the difference in mean \rsm\ between the predefined classifier with LSA (without operator feedback) and ML2ASR is zero:

\begin{align*}
        H_0^{(6)}: & \mu_{b, r,\text{LSA}} = \mu_{b, r,\text{ML2ASR}}
\end{align*}

\end{itemize}

Like previous cases, we ran multiple tests for the normality of distributions by the Anderson-Darling method. Table~\ref{tab: normality test fig 25} shows the results and indicates all tests have been rejected (with a significance level of 0.05).


\begin{table}[h]
\center
\begin{adjustbox}{max width=\textwidth}
\begin{tabular}{|c|c|c|}
\hline
 Approach & \begin{tabular}[c]{@{}c@{}}p-value (a)\end{tabular}
          & \begin{tabular}[c]{@{}c@{}}p-value (b)\end{tabular} \\ \hhline{===}
ML2ASR &   \reject{0.000} & \reject{0.000} \\ \hline
LSA &   \reject{0.000} & \reject{0.000} \\ \hline
LSA with operator &   \reject{0.000} & \reject{0.000} \\ \hline
\end{tabular}
\end{adjustbox}
\caption{\re{Normality tests for distributions in subfigures of Figure~\ref{fig: rsm total}, by Anderson-Darling test method }}
\label{tab: normality test fig 25}
\end{table}

Based on rejection of all normality tests, we used the Spearman correlation method to test the dependency (as in previous cases). Test results in Table~\ref{tab: dependency test fig 25} indicate dependency tests for all pairs were rejected with a significance level of 0.05.

\begin{table}[h]
\center
\begin{adjustbox}{max width=\textwidth}
\begin{tabular}{|c|c|c|}
\hline
 Approach & \begin{tabular}[c]{@{}c@{}}p-value (a)\end{tabular}
          & \begin{tabular}[c]{@{}c@{}}p-value (b)\end{tabular}\\ \hhline{===}
(ML2ASR, LSA) &   \reject{0.000} & \reject{0.000} \\ \hline
(ML2ASR, LSA with operator) &   \reject{0.000} & \reject{0.000}\\ \hline
(LSA, LSA with operator) &   \reject{0.000} & \reject{0.000} \\ \hline
\end{tabular}
\end{adjustbox}
\caption{\re{Dependency tests for distributions in subfigures of Figure~\ref{fig: rsm total}, by Spearman correlation test method}}
\label{tab: dependency test fig 25}
\end{table}

We tested the hypotheses with an appropriate test method based on the normality and dependency test results; see Table~\ref{tab: hypotheses test fig 25}.

% \begin{table}[h]
% \center
% \begin{adjustbox}{max width=\textwidth}
% \begin{tabular}{|c|c|c|}
% \hline
%  Hypothesis & p-value & Test method \\ \hhline{===}
% \begin{tabular}[c]{@{}c@{}}
% $H_0: \mu_{a, r,\text{LSA with operator}} = \mu_{a,r,\text{ML2ASR}}$ \\
%         $H_1: \mu_{a, r,\text{LSA with operator}} < \mu_{a, r,\text{ML2ASR}}$\end{tabular}& \reject{0.000} & Mann-Whitney U  \\ \hhline{===}
% \begin{tabular}[c]{@{}c@{}}
% $H_0: \mu_{a, r,\text{LSA with operator}} = \mu_{a,r,\text{LSA}}$ \\
%         $H_1: \mu_{a, r,\text{LSA with operator}} < \mu_{a, r,\text{LSA}}$\end{tabular}& \reject{0.000} & Mann-Whitney U  \\ \hhline{===}
% \begin{tabular}[c]{@{}c@{}}
% $H_0: \mu_{b, r,\text{LSA with operator}} = \mu_{b,r,\text{ML2ASR}}$ \\
%         $H_1: \mu_{b, r,\text{LSA with operator}} < \mu_{b, r,\text{ML2ASR}}$\end{tabular}& \reject{0.000} & Mann-Whitney U  \\ \hhline{===}
% \begin{tabular}[c]{@{}c@{}}
% $H_0: \mu_{b, r,\text{LSA with operator}} = \mu_{b,r,\text{LSA}}$ \\
%         $H_1: \mu_{b, r,\text{LSA with operator}} < \mu_{b, r,\text{LSA}}$\end{tabular}& \reject{0.000} & Mann-Whitney U  \\ \hhline{===}

% \end{tabular}
% \end{adjustbox}
% \caption{\re{Test results for all mentioned hypotheses for Figure~\ref{fig: utility total for class appearnces}, separated by double horizontal lines.}}
% \end{table}

\begin{table}[h]
\center
\begin{adjustbox}{max width=\textwidth}
\begin{tabular}{|c|c|c|c|}
\hline
\multicolumn{2}{|c|}{Hypothesis}  & p-value & Test method \\ \hhline{====}
\multicolumn{2}{|l|}{\begin{tabular}[c]{@{}c@{}}
$H_0^{(1)}: \mu_{a, r,\text{LSA with operator}} = \mu_{a,r,\text{ML2ASR}}$ \\
        $H_1^{(1)}: \mu_{a, r,\text{LSA with operator}} < \mu_{a, r,\text{ML2ASR}}$\end{tabular}}& \reject{0.000} & Mann-Whitney U  \\ \hhline{====}
\multicolumn{2}{|l|}{\begin{tabular}[c]{@{}c@{}}
$H_0^{(2)}: \mu_{a, r,\text{LSA with operator}} = \mu_{a,r,\text{LSA}}$ \\
        $H_1^{(2)}: \mu_{a, r,\text{LSA with operator}} < \mu_{a, r,\text{LSA}}$\end{tabular}}& \reject{0.000} & Mann-Whitney U  \\ \hhline{====}
\multicolumn{2}{|l|}{
$H_0^{(3)}:  \mu_{a, r,\text{LSA}} = \mu_{a, r,\text{ML2ASR}}$}& \accept{0.472} & Mann-Whitney U  \\ \hhline{====}
\multicolumn{2}{|l|}{\begin{tabular}[c]{@{}c@{}}
$H_0^{(4)}: \mu_{b, r,\text{LSA with operator}} = \mu_{b,r,\text{ML2ASR}}$ \\
        $H_1^{(4)}: \mu_{b, r,\text{LSA with operator}} < \mu_{b, r,\text{ML2ASR}}$\end{tabular}}& \reject{0.000} & Mann-Whitney U  \\ \hhline{====}
\multicolumn{2}{|l|}{\begin{tabular}[c]{@{}c@{}}
$H_0^{(5)}: \mu_{a, r,\text{LSA with operator}} = \mu_{a,r,\text{LSA}}$ \\
        $H_1^{(5)}: \mu_{a, r,\text{LSA with operator}} < \mu_{a, r,\text{LSA}}$\end{tabular}}& \reject{0.000} & Mann-Whitney U  \\ \hhline{====}
\multicolumn{2}{|l|}{
$H_0^{(6)}:  \mu_{b, r,\text{LSA}} = \mu_{b, r,\text{ML2ASR}}$}& \accept{0.441} & Mann-Whitney U  \\ \hline
\end{tabular}
\end{adjustbox}
\caption{\re{Test results for all mentioned hypotheses for Figure~\ref{fig: rsm total}, separated by double horizontal lines.}}
\label{tab: hypotheses test fig 25}
\end{table}


%%%%%%%%%%%%%%%%%%%%%%%%%%%%  Total Figures   %%%%%%%%%%%%%%%%%%%%%%%%%%%%%%%%%%%%%%%%

\subsection{ Impact of The Operator Feedback on Utilities And \rsm\ in All Scenarios 
 (Figure~\ref{fig: rsm total total})}
\label{sec: appendix fig 26}
Figure~\ref{fig: rsm total total} illustrates the impact of the operator feedback on utilities and \rsm\ in all scenarios.
We have the following set of null hypotheses and their alternatives related to this figure:

\begin{itemize}

 \item The difference in mean utility between the evolving classifier with LSA and operator feedback, and the pre-defined classifier with LSA is zero or (alternatively) greater than zero:

\begin{align*}
        H_0^{(1)}: & \mu_{a, u,\text{LSA with operator}} = \mu_{a, u,\text{LSA}} \\
        H_1^{(1)}: & \mu_{a, u,\text{LSA with operator}} > \mu_{a, u,\text{LSA}}
\end{align*}

\item The difference in mean \rsm\ between the evolving classifier with LSA and operator feedback, and the pre-defined classifier with LSA is zero or (alternatively) less than zero:

\begin{align*}
        H_0^{(2)}: & \mu_{b, r,\text{LSA with operator}} = \mu_{b, r,\text{LSA}} \\
        H_1^{(2)}: & \mu_{b, r,\text{LSA with operator}} < \mu_{b, r,\text{LSA}}
\end{align*}

\end{itemize}

Like previous cases, we ran multiple tests for the normality of distributions by the Anderson-Darling method. The following table shows the results and indicates all tests have been rejected (with a significance level of 0.05).


\begin{table}[h]
\center
\begin{adjustbox}{max width=\textwidth}
\begin{tabular}{|c|c|c|}
\hline
 Approach & \begin{tabular}[c]{@{}c@{}}p-value (a)\end{tabular}
          & \begin{tabular}[c]{@{}c@{}}p-value (b)\end{tabular} \\ \hhline{===}
LSA &   \reject{0.000} & \reject{0.000} \\ \hline
LSA with operator &   \reject{0.000} & \reject{0.000} \\ \hline
\end{tabular}
\end{adjustbox}
\caption{\re{Normality tests for distributions in subfigures of Figure~\ref{fig: rsm total total}, by Anderson-Darling test method }}
\end{table}

Based on the rejection of all normality tests, we used the Spearman correlation method to test the dependency (as in previous cases). The test result in the following table indicates the dependency test for the pair was rejected with a significance level of 0.05.

\begin{table}[h]
\center
\begin{adjustbox}{max width=\textwidth}
\begin{tabular}{|c|c|c|}
\hline
 Approach & \begin{tabular}[c]{@{}c@{}}p-value (a)\end{tabular}
          & \begin{tabular}[c]{@{}c@{}}p-value (b)\end{tabular}\\ \hhline{===}
(LSA, LSA with operator) &   \reject{0.000} & \reject{0.000} \\ \hline
\end{tabular}
\end{adjustbox}
\caption{\re{Dependency tests for distributions in subfigures of Figure~\ref{fig: rsm total total}, by Spearman correlation test method}}
\end{table}

We tested the hypotheses with an appropriate test method based on the normality and dependency test results; see the following table.

\begin{table}[h]
\center
\begin{adjustbox}{max width=\textwidth}
\begin{tabular}{|c|c|c|}
\hline
 Hypothesis & p-value & Test method \\ \hhline{===}
\begin{tabular}[c]{@{}c@{}}
$H_0^{(1)}: \mu_{a, u,\text{LSA with operator}} = \mu_{a,u,\text{ML2ASR}}$ \\
        $H_1^{(1)}: \mu_{a, u,\text{LSA with operator}} < \mu_{a, u,\text{ML2ASR}}$\end{tabular}& \reject{0.000} & Mann-Whitney U  \\ \hhline{===}
\begin{tabular}[c]{@{}c@{}}
$H_0^{(2)}: \mu_{b, r,\text{LSA with operator}} = \mu_{b,r,\text{LSA}}$ \\
        $H_1^{(2)}: \mu_{b, r,\text{LSA with operator}} < \mu_{b, r,\text{LSA}}$\end{tabular}& \reject{0.000} & Mann-Whitney U  \\ \hline

\end{tabular}
\end{adjustbox}
\caption{\re{Test results for all mentioned hypotheses for Figure~\ref{fig: rsm total total}, separated by double horizontal lines.}}
\end{table}

%}
% <-------------------------------------------------------------------------->

% \begin{table}[h]
% \center
% \begin{subtable}[t]{0.3\textwidth}
% \center
% \begin{tabular}{|l|r|}
% \hline
% \re{Hypothesis}                                          & \re{p-value} \\ \hline
% \re{$W < X$} & \re{$0.987$} \\ \hline
% \re{$W < Y$} & \re{$1.000$} \\ \hline
% \re{$W < Z$} & \re{$0.996$} \\ \hline
% \re{$X = Y$} & \re{$0.107$} \\ \hline
% \re{$X = Z$} & \re{$0.471$} \\ \hline
% \re{$Y = Z$} & \re{$0.088$} \\ \hline
% \end{tabular}
% \caption{}
% \label{tab:table fig 18_a}
% \end{subtable}
% \begin{subtable}[t]{0.3\textwidth}
% \center
% \begin{tabular}{|l|r|}
% \hline
% \re{Hypothesis}                                          & \re{p-value} \\ \hline
% \re{$W < X,Y$} & \re{$1.000$} \\ \hline
% \re{$W > Z$} & \re{$0.997$} \\ \hline
% \re{$X = Y$} & \re{$0.108$} \\ \hline
% \re{$Z < X,Y$} & \re{$1.000$} \\ \hline
% \end{tabular}
% \caption{}
% \label{tab:table fig 18a_b}
% \end{subtable}
% \caption{\re{Statistical test results corresponding to groups of box-plots ((a) and (b) for groups of left and right, i.e., no drift and novel class appearance scenarios, respectively) in Figure~\ref{fig:packet loss distribution over adaptation cycles} (packet loss values). $W$, $X$, $Y$, and $Z$ indicate random variables that follow the corresponding distributions of box plots in the figure, respectively connected to the baseline, the pre-defined classifier with ML2ASR, the pre-defined classifier with LSA (no operator feedback), and the evolving classifier with LSA and operator feedback. }} 
% \label{tab:table fig 18a}
% \end{table}

% \begin{table}[h]
% \center
% \begin{subtable}[t]{0.3\textwidth}
% \begin{tabular}{|l|r|}
% \hline
% \re{Hypothesis}                                          & \re{p-value} \\ \hline
% \re{$\mathcal{D}_1 < \mathcal{D}_2$} & \re{$0.987$} \\ \hline
% \re{$\mathcal{D}_1 < \mathcal{D}_3$} & \re{$1.000$} \\ \hline
% \re{$\mathcal{D}_1 < \mathcal{D}_4$} & \re{$0.996$} \\ \hline
% \re{$\mathcal{D}_2 = \mathcal{D}_3$} & \re{$0.107$} \\ \hline
% \re{$\mathcal{D}_2 = \mathcal{D}_4$} & \re{$0.471$} \\ \hline
% \re{$\mathcal{D}_4 = \mathcal{D}_3$} & \re{$0.088$} \\ \hline
% \end{tabular}
% \caption{}
% \label{tab:table fig 18_a}
% \end{subtable}
% \begin{subtable}[t]{0.3\textwidth}
% \begin{tabular}{|l|r|}
% \hline
% \re{Hypothesis}                                          & \re{p-value} \\ \hline
% \re{$\mathcal{D}_1 < \mathcal{D}_2, \mathcal{D}_3$} & \re{$1.000$} \\ \hline
% \re{$\mathcal{D}_1 > \mathcal{D}_4$} & \re{$0.997$} \\ \hline
% \re{$\mathcal{D}_2 = \mathcal{D}_3$} & \re{$0.108$} \\ \hline
% \re{$\mathcal{D}_4 < \mathcal{D}_2, \mathcal{D}_3$} & \re{$1.000$} \\ \hline
% \end{tabular}
% \caption{}
% \label{tab:table fig 18a_b}
% \end{subtable}
% \caption{\re{Statistical test results corresponding to groups of box-plots ((a) and (b) for groups of left and right, respectively) in Figure~\ref{fig:packet loss distribution over adaptation cycles} distribution over adaptation cycles. $\mathcal{D}_1$, $\mathcal{D}_2$, $\mathcal{D}_3$, and $\mathcal{D}_4$ denote distributions from left to right in each group, respectively.}} 
% \label{tab:table fig 18a}
% \end{table}

% <-------------------------------------------------------------------------->

% \begin{table}[h]
% \center
% \begin{subtable}[t]{0.3\textwidth}
% \center
% \begin{tabular}{|l|r|}
% \hline
% \re{Hypothesis}                                          & \re{p-value} \\ \hline
% \re{$W > X$} & \re{$0.129$} \\ \hline
% \re{$W < Y$} & \re{$0.999$} \\ \hline
% \re{$W > Z$} & \re{$0.472$} \\ \hline
% \re{$X < Y$} & \re{$0.996$} \\ \hline
% \re{$X < Z$} & \re{$0.214$} \\ \hline
% \re{$Y > Z$} & \re{$0.999$} \\ \hline
% \end{tabular}
% \caption{}
% \label{tab:table fig 18b_a}
% \end{subtable}
% \begin{subtable}[t]{0.3\textwidth}
% \center
% \begin{tabular}{|l|r|}
% \hline
% \re{Hypothesis}                                          & \re{p-value} \\ \hline
% \re{$W < X, Y$} & \re{$1.000$} \\ \hline
% \re{$W > Z$} & \re{$0.616$} \\ \hline
% \re{$X = Y$} & \re{$0.362$} \\ \hline
% \re{$Z < X, Y$} & \re{$1.000$} \\ \hline
% \end{tabular}
% \caption{}
% \label{tab:table fig 18b_b}
% \end{subtable}
% \caption{\re{Statistical test results corresponding to groups of box-plots ((a) and (b) for groups of left and right, i.e., no drift and novel class appearance scenarios, respectively) in Figure~\ref{fig:energy consumption distribution over adaptation cycles} (energy consumption values). $W$, $X$, $Y$, and $Z$ indicate random variables that follow the corresponding distributions of box plots in the figure, respectively connected to the baseline, the pre-defined classifier with ML2ASR, the pre-defined classifier with LSA (no operator feedback), and the evolving classifier with LSA and operator feedback.} }
% \label{tab:table fig 18b}
% \end{table}

% \re{Hypothesis}                                          & \re{p-value} \\ \hline
% \re{$\mathcal{D}_1 > \mathcal{D}_2$} & \re{$0.129$} \\ \hline
% \re{$\mathcal{D}_1 < \mathcal{D}_3$} & \re{$0.999$} \\ \hline
% \re{$\mathcal{D}_1 > \mathcal{D}_4$} & \re{$0.472$} \\ \hline
% \re{$\mathcal{D}_2 < \mathcal{D}_3$} & \re{$0.996$} \\ \hline
% \re{$\mathcal{D}_2 < \mathcal{D}_4$} & \re{$0.214$} \\ \hline
% \re{$\mathcal{D}_3 > \mathcal{D}_4$} & \re{$0.999$} \\ \hline
% \end{tabular}
% \caption{}
% \label{tab:table fig 18b_a}
% \end{subtable}
% \begin{subtable}[t]{0.3\textwidth}
% \begin{tabular}{|l|r|}
% \hline
% \re{Hypothesis}                                          & \re{p-value} \\ \hline
% \re{$\mathcal{D}_1 < \mathcal{D}_2, \mathcal{D}_3$} & \re{$1.000$} \\ \hline
% \re{$\mathcal{D}_1 > \mathcal{D}_4$} & \re{$0.616$} \\ \hline
% \re{$\mathcal{D}_2 = \mathcal{D}_3$} & \re{$0.362$} \\ \hline
% \re{$\mathcal{D}_4 < \mathcal{D}_2, \mathcal{D}_3$} & \re{$1.000$} \\ \hline
% \end{tabular}
% \caption{}
% \label{tab:table fig 18b_b}
% \end{subtable}


% <-------------------------------------------------------------------------->

% \begin{table}[h]
% \center
% \begin{subtable}[t]{0.3\textwidth}
% \center
% \begin{tabular}{|l|r|}
% \hline
% \re{Hypothesis}                                          & \re{p-value} \\ \hline
% \re{$W > X$} & \re{$0.950$} \\ \hline
% \re{$W > Y$} & \re{$1.000$} \\ \hline
% \re{$W > Z$} & \re{$0.958$} \\ \hline
% \re{$X > Y$} & \re{$0.993$} \\ \hline
% \re{$X > Z$} & \re{$0.417$} \\ \hline
% \re{$Z > Y$} & \re{$0.997$} \\ \hline
% \end{tabular}
% \caption{}
% \label{tab:table fig 19_a}
% \end{subtable}
% \begin{subtable}[t]{0.3\textwidth}
% \center
% \begin{tabular}{|l|r|}
% \hline
% \re{Hypothesis}                                          & \re{p-value} \\ \hline
% \re{$W > X, Y$} & \re{$1.000$} \\ \hline
% \re{$W = Z$} & \re{$0.105$} \\ \hline
% \re{$X > Y$} & \re{$0.951$} \\ \hline
% \re{$Z > X, Y$} & \re{$1.000$} \\ \hline
% \end{tabular}
% \caption{}
% \label{tab:table fig 19_b}
% \end{subtable}
% \caption{\re{Statistical test results corresponding to groups of box-plots ((a) and (b) for groups of left and right, i.e., no drift and novel class appearance scenarios, respectively) in Figure~\ref{fig:resuls-utilities} (impact of drift of adaptation spaces on the utility of the system). $W$, $X$, $Y$, and $Z$ indicate random variables that follow the corresponding distributions of box plots in the figure, respectively connected to the baseline, the pre-defined classifier with ML2ASR, the pre-defined classifier with LSA (no operator feedback), and the evolving classifier with LSA and operator feedback.} }
% \label{tab:table fig 19}
% \end{table}

% \begin{subtable}[t]{0.3\textwidth}
% \begin{tabular}{|l|r|}
% \hline
% \re{Hypothesis}                                          & \re{p-value} \\ \hline
% \re{$\mathcal{D}_1 > \mathcal{D}_2$} & \re{$0.950$} \\ \hline
% \re{$\mathcal{D}_1 > \mathcal{D}_3$} & \re{$1.000$} \\ \hline
% \re{$\mathcal{D}_1 > \mathcal{D}_4$} & \re{$0.958$} \\ \hline
% \re{$\mathcal{D}_2 > \mathcal{D}_3$} & \re{$0.993$} \\ \hline
% \re{$\mathcal{D}_2 > \mathcal{D}_4$} & \re{$0.417$} \\ \hline
% \re{$\mathcal{D}_4 > \mathcal{D}_3$} & \re{$0.997$} \\ \hline
% \end{tabular}
% \caption{}
% \label{tab:table fig 19_a}
% \end{subtable}
% \begin{subtable}[t]{0.3\textwidth}
% \begin{tabular}{|l|r|}
% \hline
% \re{Hypothesis}                                          & \re{p-value} \\ \hline
% \re{$\mathcal{D}_1 > \mathcal{D}_2, \mathcal{D}_3$} & \re{$1.000$} \\ \hline
% \re{$\mathcal{D}_1 = \mathcal{D}_4$} & \re{$0.105$} \\ \hline
% \re{$\mathcal{D}_2 > \mathcal{D}_3$} & \re{$0.951$} \\ \hline
% \re{$\mathcal{D}_4 > \mathcal{D}_2, \mathcal{D}_3$} & \re{$1.000$} \\ \hline
% \end{tabular}
% \caption{}
% \label{tab:table fig 19_b}
% \end{subtable}

% <-------------------------------------------------------------------------->

% \begin{table}[h]
% \center
% \begin{subtable}[t]{0.3\textwidth}
% \center
% \begin{tabular}{|l|r|}
% \hline
% \re{Hypothesis}                                          & \re{p-value} \\ \hline
% \re{$X = Y$} & \re{$0.489$} \\ \hline
% \re{$X = Z$} & \re{$0.169$} \\ \hline
% \re{$Y = Z$} & \re{$0.169$} \\ \hline
% \end{tabular}
% \caption{}
% \label{tab:table fig 20_a}
% \end{subtable}
% \begin{subtable}[t]{0.3\textwidth}
% \center
% \begin{tabular}{|l|r|}
% \hline
% \re{Hypothesis}                                          & \re{p-value} \\ \hline
% \re{$X = Y$} & \re{$0.469$} \\ \hline
% \re{$X, Y > Z$}      & \re{$1.000$} \\ \hline
% \end{tabular}
% \caption{}
% \label{tab:table fig 20_b}
% \end{subtable}
% \caption{\re{Statistical test results corresponding to groups of box-plots ((a) and (b) for groups of left and right, i.e., no drift and novel class appearance scenarios, respectively) in Figure~\ref{fig: rsm improvement} (impact of drift of adaptation spaces on the RSM for different approaches). $X$, $Y$, and $Z$ indicate random variables that follow the corresponding distributions of box plots in the figure, respectively connected to the pre-defined classifier with ML2ASR, 
%  the pre-defined classifier with LSA (no operator feedback), and the evolving classifier with LSA and operator feedback.} }
% \label{tab:table fig 20}
% \end{table}

% \begin{subtable}[t]{0.3\textwidth}
% \begin{tabular}{|l|r|}
% \hline
% \re{Hypothesis}                                          & \re{p-value} \\ \hline
% \re{$\mathcal{D}_1 = \mathcal{D}_2$} & \re{$0.489$} \\ \hline
% \re{$\mathcal{D}_1 = \mathcal{D}_3$} & \re{$0.169$} \\ \hline
% \re{$\mathcal{D}_2 = \mathcal{D}_3$} & \re{$0.169$} \\ \hline
% \end{tabular}
% \caption{}
% \label{tab:table fig 20_a}
% \end{subtable}
% \begin{subtable}[t]{0.3\textwidth}
% \begin{tabular}{|l|r|}
% \hline
% \re{Hypothesis}                                          & \re{p-value} \\ \hline
% \re{$\mathcal{D}_1 = \mathcal{D}_2$} & \re{$0.469$} \\ \hline
% \re{$\mathcal{D}_1, \mathcal{D}_2 > \mathcal{D}_3$}      & \re{$1.000$} \\ \hline
% \end{tabular}
% \caption{}
% \label{tab:table fig 20_b}
% \end{subtable}

% <-------------------------------------------------------------------------->

% \begin{table}[h]
% \center
% \begin{subtable}[t]{0.3\textwidth}
% \center
% \begin{tabular}{|l|r|}
% \hline
% \re{Hypothesis}                                          & \re{p-value} \\ \hline
% \re{$W > X, Y$}      & \re{$1.000$} \\ \hline
% \re{$W > Z$} & \re{$0.951$} \\ \hline
% \re{$Z > X, Y$}      & \re{$1.000$} \\ \hline
% \re{$X = Y$}                     & \re{$0.364$} \\ \hline
% \end{tabular}
% \caption{$\langle$(B),R, G$\rangle$}
% \label{tab:table fig 21_a}
% \end{subtable}
% \begin{subtable}[t]{0.3\textwidth}
% \center
% \begin{tabular}{|l|r|}
% \hline
% \re{Hypothesis}                                          & \re{p-value} \\ \hline
% \re{$W > X, Y$}      & \re{$1.000$} \\ \hline
% \re{$W = Z$} & \re{$0.083$} \\ \hline
% \re{$Z > X, Y$}      & \re{$1.000$} \\ \hline
% \re{$X = Y$}                     & \re{$0.294$} \\ \hline
% \end{tabular}
% \caption{$\langle$(B),G, R$\rangle$}
% \label{tab:table fig 21_b}
% \end{subtable}

% \bigskip 

% \begin{subtable}[t]{0.3\textwidth}
% \center
% \begin{tabular}{|l|r|}
% \hline
% \re{Hypothesis}                                          & \re{p-value} \\ \hline
% \re{$W > X$}      & \re{$0.990$} \\ \hline
% \re{$W > Y$}      & \re{$0.997$} \\ \hline
% \re{$W = Z$} & \re{$0.234$} \\ \hline
% \re{$Z > X$}      & \re{$0.163$} \\ \hline
% \re{$Z > Y$}      & \re{$0.253$} \\ \hline
% \re{$X = Y$}                     & \re{$0.433$} \\ \hline
% \end{tabular}
% \caption{$\langle$(R),B, G$\rangle$}
% \label{tab:table fig 21_c}
% \end{subtable}
% \begin{subtable}[t]{0.3\textwidth}
% \center
% \begin{tabular}{|l|r|}
% \hline
% \re{Hypothesis}                                          & \re{p-value} \\ \hline
% \re{$W > X$}      & \re{$0.980$} \\ \hline
% \re{$W > Y$}      & \re{$0.988$} \\ \hline
% \re{$W = Z$} & \re{$0.282$} \\ \hline
% \re{$Z > X$}      & \re{$0.402$} \\ \hline
% \re{$Z > Y$}      & \re{$0.461$} \\ \hline
% \re{$X = Y$}                     & \re{$0.488$} \\ \hline
% \end{tabular}
% \caption{$\langle$(R),G, B$\rangle$}
% \label{tab:table fig 21_d}
% \end{subtable}

% \bigskip

% \begin{subtable}[t]{0.3\textwidth}
% \center
% \begin{tabular}{|l|r|}
% \hline
% \re{Hypothesis}                                          & \re{p-value} \\ \hline
% \re{$W > X, Y$}      & \re{$1.000$} \\ \hline
% \re{$W = Z$} & \re{$0.372$} \\ \hline
% \re{$Z > X, Y$}      & \re{$1.000$} \\ \hline
% \re{$X = Y$}                     & \re{$0.342$} \\ \hline
% \end{tabular}
% \caption{$\langle$(B, R),G$\rangle$}
% \label{tab:table fig 21_e}
% \end{subtable}
% \begin{subtable}[t]{0.3\textwidth}
% \center
% \begin{tabular}{|l|r|}
% \hline
% \re{Hypothesis}                                          & \re{p-value} \\ \hline
% \re{$W > X$}      & \re{$0.999$} \\ \hline
% \re{$W > Y$}      & \re{$0.998$} \\ \hline
% \re{$W > Z$} & \re{$0.997$} \\ \hline
% \re{$Z = X$}      & \re{$0.191$} \\ \hline
% \re{$Z = Y$}      & \re{$0.348$} \\ \hline
% \re{$X = Y$}                     & \re{$0.306$} \\ \hline
% \end{tabular}
% \caption{$\langle$(B,G),R$\rangle$}
% \label{tab:table fig 21_f}
% \end{subtable}

% \caption{\re{Statistical test results corresponding to subfigures in Figure~\ref{fig: utility total for class appearnces} (utility for all preference orders of stakeholders split for classes appearance orders). $W$, $X$, $Y$, and $Z$ indicate random variables that follow the corresponding distributions of box plots in the figure, respectively connected to the baseline, the pre-defined classifier with ML2ASR, the pre-defined classifier with LSA (no operator feedback), and the evolving classifier with LSA and operator feedback.}}
% \label{tab:table fig 21}
% \end{table}


% \begin{subtable}[t]{0.3\textwidth}
% \begin{tabular}{|l|r|}
% \hline
% \re{Hypothesis}                                          & \re{p-value} \\ \hline
% \re{$\mathcal{D}_1 > \mathcal{D}_2, \mathcal{D}_3$}      & \re{$1.000$} \\ \hline
% \re{$\mathcal{D}_1 > \mathcal{D}_4$} & \re{$0.951$} \\ \hline
% \re{$\mathcal{D}_4 > \mathcal{D}_2, \mathcal{D}_3$}      & \re{$1.000$} \\ \hline
% \re{$\mathcal{D}_2 = \mathcal{D}_3$}                     & \re{$0.364$} \\ \hline
% \end{tabular}
% \caption{}
% \label{tab:table fig 21_a}
% \end{subtable}
% \begin{subtable}[t]{0.3\textwidth}
% \begin{tabular}{|l|r|}
% \hline
% \re{Hypothesis}                                          & \re{p-value} \\ \hline
% \re{$\mathcal{D}_1 > \mathcal{D}_2, \mathcal{D}_3$}      & \re{$1.000$} \\ \hline
% \re{$\mathcal{D}_1 = \mathcal{D}_4$} & \re{$0.083$} \\ \hline
% \re{$\mathcal{D}_4 > \mathcal{D}_2, \mathcal{D}_3$}      & \re{$1.000$} \\ \hline
% \re{$\mathcal{D}_2 = \mathcal{D}_3$}                     & \re{$0.294$} \\ \hline
% \end{tabular}
% \caption{}
% \label{tab:table fig 21_b}
% \end{subtable}

% \bigskip 

% \begin{subtable}[t]{0.3\textwidth}
% \begin{tabular}{|l|r|}
% \hline
% \re{Hypothesis}                                          & \re{p-value} \\ \hline
% \re{$\mathcal{D}_1 > \mathcal{D}_2$}      & \re{$0.990$} \\ \hline
% \re{$\mathcal{D}_1 > \mathcal{D}_3$}      & \re{$0.997$} \\ \hline
% \re{$\mathcal{D}_1 = \mathcal{D}_4$} & \re{$0.234$} \\ \hline
% \re{$\mathcal{D}_4 > \mathcal{D}_2$}      & \re{$0.163$} \\ \hline
% \re{$\mathcal{D}_4 > \mathcal{D}_3$}      & \re{$0.253$} \\ \hline
% \re{$\mathcal{D}_2 = \mathcal{D}_3$}                     & \re{$0.433$} \\ \hline
% \end{tabular}
% \caption{}
% \label{tab:table fig 21_c}
% \end{subtable}
% \begin{subtable}[t]{0.3\textwidth}
% \begin{tabular}{|l|r|}
% \hline
% \re{Hypothesis}                                          & \re{p-value} \\ \hline
% \re{$\mathcal{D}_1 > \mathcal{D}_2$}      & \re{$0.980$} \\ \hline
% \re{$\mathcal{D}_1 > \mathcal{D}_3$}      & \re{$0.988$} \\ \hline
% \re{$\mathcal{D}_1 = \mathcal{D}_4$} & \re{$0.282$} \\ \hline
% \re{$\mathcal{D}_4 > \mathcal{D}_2$}      & \re{$0.402$} \\ \hline
% \re{$\mathcal{D}_4 > \mathcal{D}_3$}      & \re{$0.461$} \\ \hline
% \re{$\mathcal{D}_2 = \mathcal{D}_3$}                     & \re{$0.488$} \\ \hline
% \end{tabular}
% \caption{}
% \label{tab:table fig 21_d}
% \end{subtable}

% \bigskip

% \begin{subtable}[t]{0.3\textwidth}
% \begin{tabular}{|l|r|}
% \hline
% \re{Hypothesis}                                          & \re{p-value} \\ \hline
% \re{$\mathcal{D}_1 > \mathcal{D}_2, \mathcal{D}_3$}      & \re{$1.000$} \\ \hline
% \re{$\mathcal{D}_1 = \mathcal{D}_4$} & \re{$0.372$} \\ \hline
% \re{$\mathcal{D}_4 > \mathcal{D}_2, \mathcal{D}_3$}      & \re{$1.000$} \\ \hline
% \re{$\mathcal{D}_2 = \mathcal{D}_3$}                     & \re{$0.342$} \\ \hline
% \end{tabular}
% \caption{}
% \label{tab:table fig 21_e}
% \end{subtable}
% \begin{subtable}[t]{0.3\textwidth}
% \begin{tabular}{|l|r|}
% \hline
% \re{Hypothesis}                                          & \re{p-value} \\ \hline
% \re{$\mathcal{D}_1 > \mathcal{D}_2$}      & \re{$0.999$} \\ \hline
% \re{$\mathcal{D}_1 > \mathcal{D}_3$}      & \re{$0.998$} \\ \hline
% \re{$\mathcal{D}_1 > \mathcal{D}_4$} & \re{$0.997$} \\ \hline
% \re{$\mathcal{D}_4 = \mathcal{D}_2$}      & \re{$0.191$} \\ \hline
% \re{$\mathcal{D}_4 = \mathcal{D}_3$}      & \re{$0.348$} \\ \hline
% \re{$\mathcal{D}_2 = \mathcal{D}_3$}                     & \re{$0.306$} \\ \hline
% \end{tabular}
% \caption{}
% \label{tab:table fig 21_f}
% \end{subtable}
% <-------------------------------------------------------------------------->

% \begin{table}[h]
% \center
% \begin{subtable}[t]{0.3\textwidth}
% \center
% \begin{tabular}{|l|r|}
% \hline
% \re{Hypothesis}                                          & \re{p-value} \\ \hline
% \re{$X = Y$}      & \re{$0.494$} \\ \hline
% \re{$X, Y > Z$} & \re{$1.000$} \\ \hline
% \end{tabular}
% \caption{$\langle$(B),R, G$\rangle$}
% \label{tab:table fig 22_a}
% \end{subtable}
% \begin{subtable}[t]{0.3\textwidth}
% \center
% \begin{tabular}{|l|r|}
% \hline
% \re{Hypothesis}                                          & \re{p-value} \\ \hline
% \re{$X = Y$}      & \re{$0.330$} \\ \hline
% \re{$X > Z$} & \re{$0.980$} \\ \hline
% \re{$Y > Z$} & \re{$0.972$} \\ \hline
% \end{tabular}
% \caption{$\langle$(B),G, R$\rangle$}
% \label{tab:table fig 22_b}
% \end{subtable}

% \bigskip 

% \begin{subtable}[t]{0.3\textwidth}
% \center
% \begin{tabular}{|l|r|}
% \hline
% \re{Hypothesis}                                          & \re{p-value} \\ \hline
% \re{$X = Y$}      & \re{$0.411$} \\ \hline
% \re{$X> Z$} & \re{$0.990$} \\ \hline
% \re{$Y> Z$} & \re{$0.991$} \\ \hline
% \end{tabular}
% \caption{$\langle$(R),B, G$\rangle$}
% \label{tab:table fig 22_c}
% \end{subtable}
% \begin{subtable}[t]{0.3\textwidth}
% \center
% \begin{tabular}{|l|r|}
% \hline
% \re{Hypothesis}                                          & \re{p-value} \\ \hline
% \re{$X = Y$}      & \re{$0.463$} \\ \hline
% \re{$X> Z$} & \re{$0.987$} \\ \hline
% \re{$Y> Z$} & \re{$0.988$} \\ \hline
% \end{tabular}
% \caption{$\langle$(R),G, B$\rangle$}
% \label{tab:table fig 22_d}
% \end{subtable}

% \bigskip

% \begin{subtable}[t]{0.3\textwidth}
% \center
% \begin{tabular}{|l|r|}
% \hline
% \re{Hypothesis}                                          & \re{p-value} \\ \hline
% \re{$X = Y$}      & \re{$0.424$} \\ \hline
% \re{$X, Y > Z$} & \re{$1.000$} \\ \hline
% \end{tabular}
% \caption{$\langle$(B,R), G$\rangle$}
% \label{tab:table fig 22_e}
% \end{subtable}
% \begin{subtable}[t]{0.3\textwidth}
% \center
% \begin{tabular}{|l|r|}
% \hline
% \re{Hypothesis}                                          & \re{p-value} \\ \hline
% \re{$X = Y$}      & \re{$0.392$} \\ \hline
% \re{$X = Z$} & \re{$0.447$} \\ \hline
% \re{$Y = Z$} & \re{$0.341$} \\ \hline
% \end{tabular}
% \caption{$\langle$(B,G),R$\rangle$}
% \label{tab:table fig 22_f}
% \end{subtable}



% \caption{\re{Statistical test results corresponding to subfigures in Figure~\ref{fig: rsm total for class appearnces} (RSM values for all preference orders of stakeholders split for classes appearance order). $X$, $Y$, and $Z$ indicate random variables that follow the corresponding distributions of box plots in the figure, respectively connected to the pre-defined classifier with ML2ASR, the pre-defined classifier with LSA (no operator feedback), and the evolving classifier with LSA and operator feedback.}}
% \label{tab:table fig 22}
% \end{table}

% \begin{subtable}[t]{0.3\textwidth}
% \begin{tabular}{|l|r|}
% \hline
% \re{Hypothesis}                                          & \re{p-value} \\ \hline
% \re{$\mathcal{D}_1 = \mathcal{D}_2$}      & \re{$0.494$} \\ \hline
% \re{$\mathcal{D}_1, \mathcal{D}_2 > \mathcal{D}_3$} & \re{$1.000$} \\ \hline
% \end{tabular}
% \caption{}
% \label{tab:table fig 22_a}
% \end{subtable}
% \begin{subtable}[t]{0.3\textwidth}
% \begin{tabular}{|l|r|}
% \hline
% \re{Hypothesis}                                          & \re{p-value} \\ \hline
% \re{$\mathcal{D}_1 = \mathcal{D}_2$}      & \re{$0.330$} \\ \hline
% \re{$\mathcal{D}_1 > \mathcal{D}_3$} & \re{$0.980$} \\ \hline
% \re{$\mathcal{D}_2 > \mathcal{D}_3$} & \re{$0.972$} \\ \hline
% \end{tabular}
% \caption{}
% \label{tab:table fig 22_b}
% \end{subtable}

% \bigskip 

% \begin{subtable}[t]{0.3\textwidth}
% \begin{tabular}{|l|r|}
% \hline
% \re{Hypothesis}                                          & \re{p-value} \\ \hline
% \re{$\mathcal{D}_1 = \mathcal{D}_2$}      & \re{$0.411$} \\ \hline
% \re{$\mathcal{D}_1> \mathcal{D}_3$} & \re{$0.990$} \\ \hline
% \re{$\mathcal{D}_2> \mathcal{D}_3$} & \re{$0.991$} \\ \hline
% \end{tabular}
% \caption{}
% \label{tab:table fig 22_c}
% \end{subtable}
% \begin{subtable}[t]{0.3\textwidth}
% \begin{tabular}{|l|r|}
% \hline
% \re{Hypothesis}                                          & \re{p-value} \\ \hline
% \re{$\mathcal{D}_1 = \mathcal{D}_2$}      & \re{$0.463$} \\ \hline
% \re{$\mathcal{D}_1> \mathcal{D}_3$} & \re{$0.987$} \\ \hline
% \re{$\mathcal{D}_2> \mathcal{D}_3$} & \re{$0.988$} \\ \hline
% \end{tabular}
% \caption{}
% \label{tab:table fig 22_d}
% \end{subtable}

% \bigskip

% \begin{subtable}[t]{0.3\textwidth}
% \begin{tabular}{|l|r|}
% \hline
% \re{Hypothesis}                                          & \re{p-value} \\ \hline
% \re{$\mathcal{D}_1 = \mathcal{D}_2$}      & \re{$0.424$} \\ \hline
% \re{$\mathcal{D}_1, \mathcal{D}_2 > \mathcal{D}_3$} & \re{$1.000$} \\ \hline
% \end{tabular}
% \caption{}
% \label{tab:table fig 22_e}
% \end{subtable}
% \begin{subtable}[t]{0.3\textwidth}
% \begin{tabular}{|l|r|}
% \hline
% \re{Hypothesis}                                          & \re{p-value} \\ \hline
% \re{$\mathcal{D}_1 = \mathcal{D}_2$}      & \re{$0.392$} \\ \hline
% \re{$\mathcal{D}_1 = \mathcal{D}_3$} & \re{$0.447$} \\ \hline
% \re{$\mathcal{D}_2 = \mathcal{D}_3$} & \re{$0.341$} \\ \hline
% \end{tabular}
% \caption{}
% \label{tab:table fig 22_f}
% \end{subtable}

% <-------------------------------------------------------------------------->

% \begin{table}[h]
% \center
% \begin{subtable}[t]{0.48\textwidth}
% \center
% \begin{tabular}{|l|r|}
% \hline
% \re{Hypothesis}                                          & \re{p-value} \\ \hline
% \re{$W > X, Y$}      & \re{$1.000$} \\ \hline
% \re{$W = Z$} & \re{$0.086$} \\ \hline
% \re{$X = Y$} & \re{$0.472$} \\ \hline
% \re{$Z > X, Y$} & \re{$1.000$} \\ \hline
% \end{tabular}
% \caption{$\langle$``less packet loss'', ``less energy consumption''$\rangle$}
% \label{tab:table fig 23_a}
% \end{subtable}
% \begin{subtable}[t]{0.48\textwidth}
% \center
% \begin{tabular}{|l|r|}
% \hline
% \re{Hypothesis}                                          & \re{p-value} \\ \hline
% \re{$W > X, Y, Z$}      & \re{$1.000$} \\ \hline
% \re{$X = Y$} & \re{$0.394$} \\ \hline
% \re{$Z > X, Y$} & \re{$1.000$} \\ \hline
% \end{tabular}
% \caption{$\langle$``less energy consumption'', ``less packet loss''$\rangle$}
% \label{tab:table fig 23_b}
% \end{subtable}
% \caption{\re{Statistical test results corresponding to subfigures in Figure~\ref{fig: utility total} (utility for all class appearance order scenarios split for preference order of stakeholders). $W$, $X$, $Y$, and $Z$ indicate random variables that follow the corresponding distributions of box plots in the figure, respectively connected to the baseline, the pre-defined classifier with ML2ASR, the pre-defined classifier with LSA (no operator feedback), and the evolving classifier with LSA and operator feedback.} }
% \label{tab:table fig 23}
% \end{table}


% \begin{subtable}[t]{0.3\textwidth}
% \begin{tabular}{|l|r|}
% \hline
% \re{Hypothesis}                                          & \re{p-value} \\ \hline
% \re{$\mathcal{D}_1 > \mathcal{D}_2, \mathcal{D}_3$}      & \re{$1.000$} \\ \hline
% \re{$\mathcal{D}_1 = \mathcal{D}_4$} & \re{$0.086$} \\ \hline
% \re{$\mathcal{D}_2 = \mathcal{D}_3$} & \re{$0.472$} \\ \hline
% \re{$\mathcal{D}_4 > \mathcal{D}_2, \mathcal{D}_3$} & \re{$1.000$} \\ \hline
% \end{tabular}
% \caption{$\langle$``less packet loss'', ``less energy consumption''$\rangle$}
% \label{tab:table fig 23_a}
% \end{subtable}
% \begin{subtable}[t]{0.3\textwidth}
% \begin{tabular}{|l|r|}
% \hline
% \re{Hypothesis}                                          & \re{p-value} \\ \hline
% \re{$\mathcal{D}_1 > \mathcal{D}_2, \mathcal{D}_3, \mathcal{D}_4$}      & \re{$1.000$} \\ \hline
% \re{$\mathcal{D}_2 = \mathcal{D}_3$} & \re{$0.394$} \\ \hline
% \re{$\mathcal{D}_4 > \mathcal{D}_2, \mathcal{D}_3$} & \re{$1.000$} \\ \hline
% \end{tabular}
% \caption{$\langle$``less energy consumption'', ``less packet loss''$\rangle$}
% \label{tab:table fig 23_b}
% \end{subtable}
% <-------------------------------------------------------------------------->

% \begin{table}[h]
% \center
% \begin{subtable}[t]{0.48\textwidth}
% \center
% \begin{tabular}{|l|r|}
% \hline
% \re{Hypothesis}                                          & \re{p-value} \\ \hline
% \re{$X = Y$} & \re{$0.472$} \\ \hline
% \re{$X, Y > Z$}      & \re{$1.000$} \\ \hline
% \end{tabular}
% \caption{$\langle$``less packet loss'', ``less energy consumption''$\rangle$}
% \label{tab:table fig 24_a}
% \end{subtable}
% \begin{subtable}[t]{0.48\textwidth}
% \center
% \begin{tabular}{|l|r|}
% \hline
% \re{Hypothesis}                                          & \re{p-value} \\ \hline
% \re{$X = Y$} & \re{$0.441$} \\ \hline
% \re{$X, Y > Z$}      & \re{$1.000$} \\ \hline
% \end{tabular}
% \caption{$\langle$``less energy consumption'', ``less packet loss''$\rangle$}
% \label{tab:table fig 24_b}
% \end{subtable}
% \caption{\re{Statistical test results corresponding to subfigures in Figure~\ref{fig: rsm total} (RSM values for all class appearance order scenarios split for preference order of stakeholders). $X$, $Y$, and $Z$ indicate random variables that follow the corresponding distributions of box plots in the figure, respectively connected to the pre-defined classifier with ML2ASR, the pre-defined classifier with LSA (no operator feedback), and the evolving classifier with LSA and operator feedback.} }
% \label{tab:table fig 24}
% \end{table}


% \begin{subtable}[t]{0.3\textwidth}
% \begin{tabular}{|l|r|}
% \hline
% \re{Hypothesis}                                          & \re{p-value} \\ \hline
% \re{$\mathcal{D}_1 = \mathcal{D}_2$} & \re{$0.472$} \\ \hline
% \re{$\mathcal{D}_1, \mathcal{D}_2 > \mathcal{D}_3$}      & \re{$1.000$} \\ \hline
% \end{tabular}
% \caption{$\langle$``less packet loss'', ``less energy consumption''$\rangle$}
% \label{tab:table fig 24_a}
% \end{subtable}
% \begin{subtable}[t]{0.3\textwidth}
% \begin{tabular}{|l|r|}
% \hline
% \re{Hypothesis}                                          & \re{p-value} \\ \hline
% \re{$\mathcal{D}_1 = \mathcal{D}_2$} & \re{$0.441$} \\ \hline
% \re{$\mathcal{D}_1, \mathcal{D}_2 > \mathcal{D}_3$}      & \re{$1.000$} \\ \hline
% \end{tabular}
% \caption{$\langle$``less energy consumption'', ``less packet loss''$\rangle$}
% \label{tab:table fig 24_b}
% \end{subtable}
% <-------------------------------------------------------------------------->
